# Supplementary material for: A Multiwavelength Classification and Study of Red Supergiant Candidates in NGC 6946
Source: arXiv:2303.03392 source file (2023-03-06)
Supplement: Supplementary file 1 [file appendix.tex]

\begin{figure}[hbt!]
        \centering
        \begin{minipage}{.3\textwidth}
            \centering
            \includegraphics[width=\textwidth]{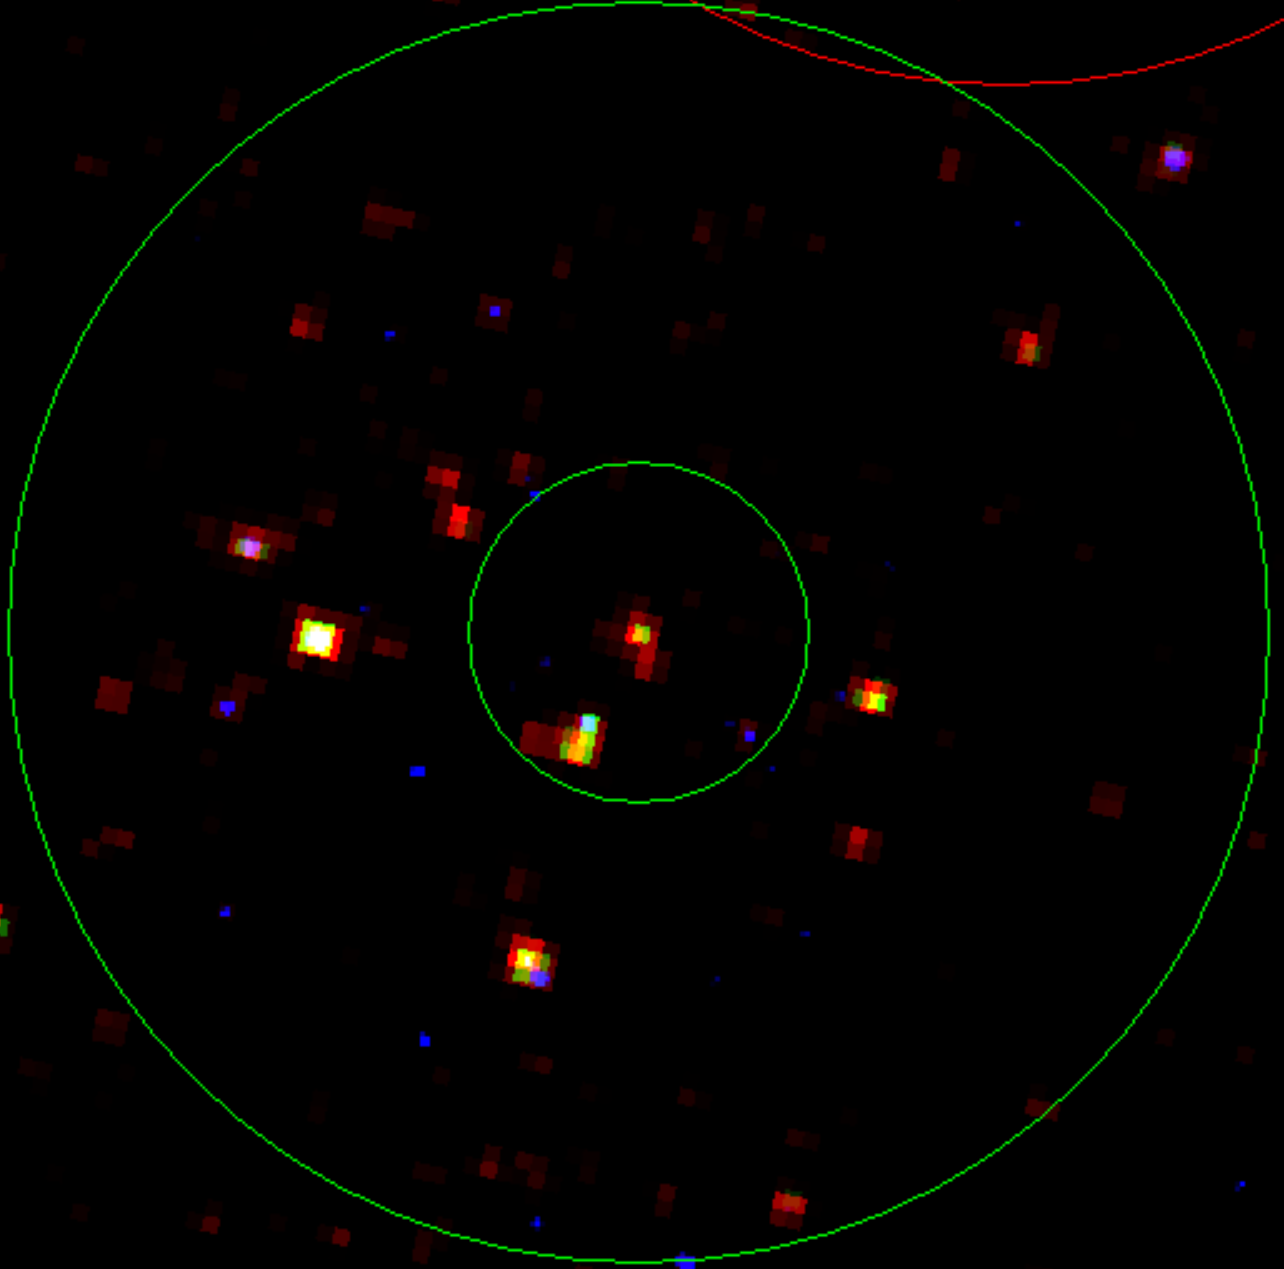}
            \\ RSG 3335 - 13 Myr
        \end{minipage}
        \begin{minipage}{.3\textwidth}
            \centering
            \includegraphics[width=\textwidth]{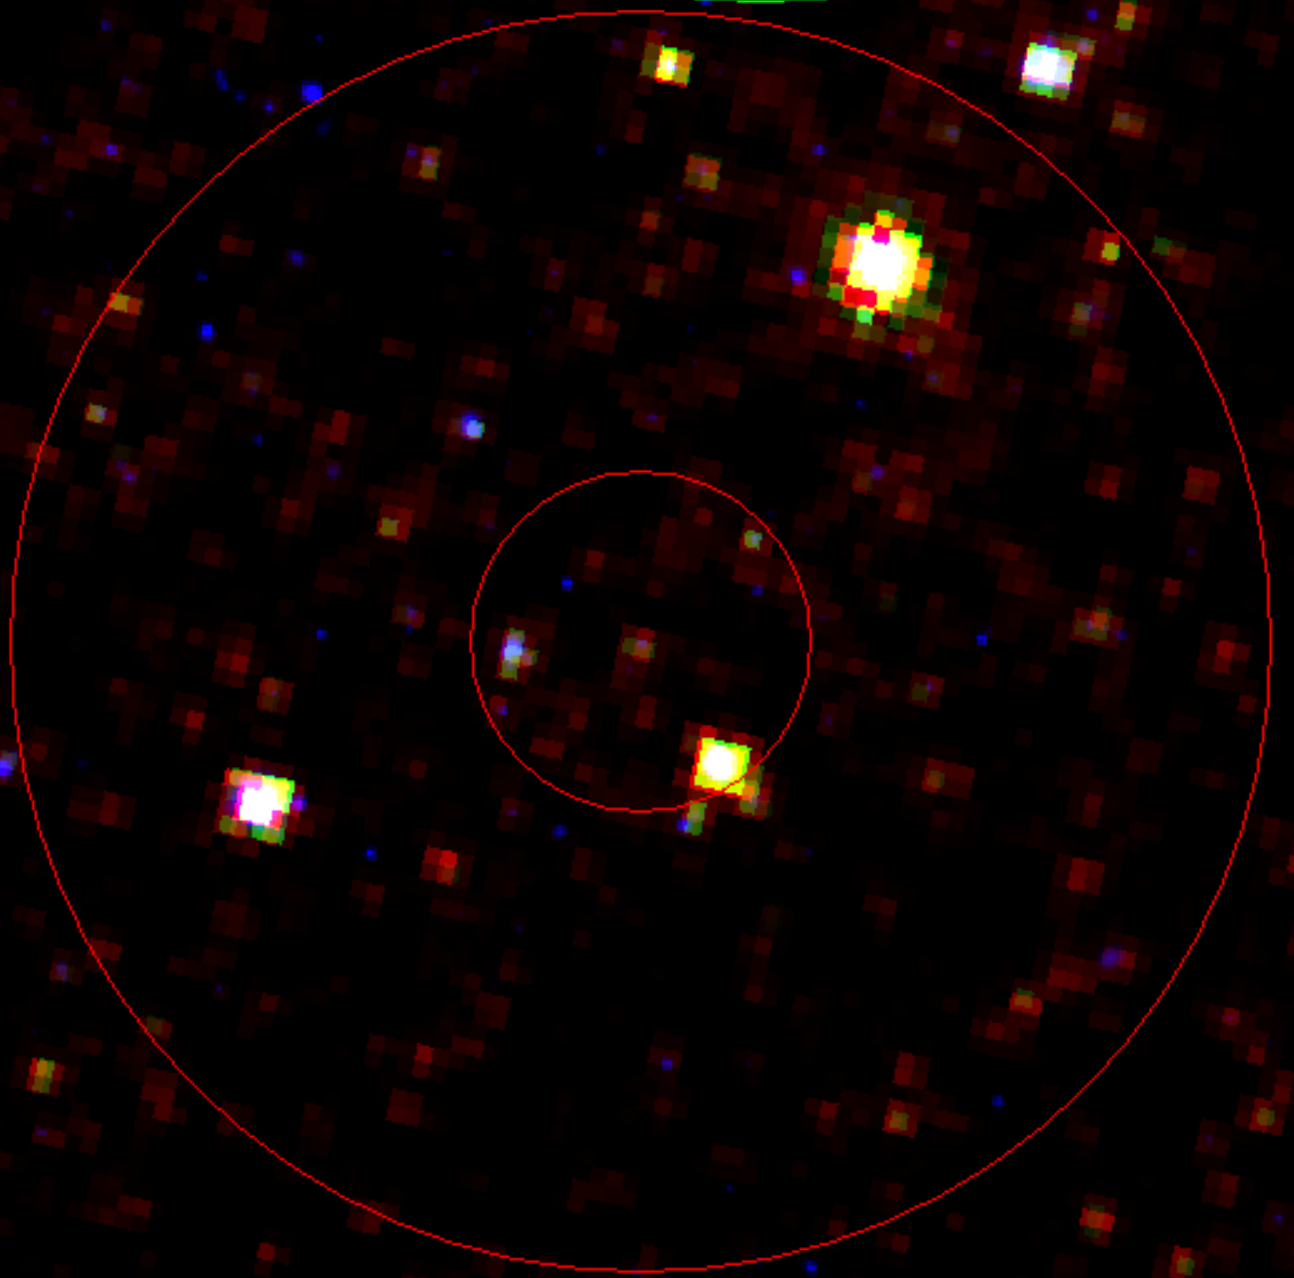}
            \\ RSG 4623 - 29 Myr
        \end{minipage}
        \begin{minipage}{.3\textwidth}
            \centering
            \includegraphics[width=\textwidth]{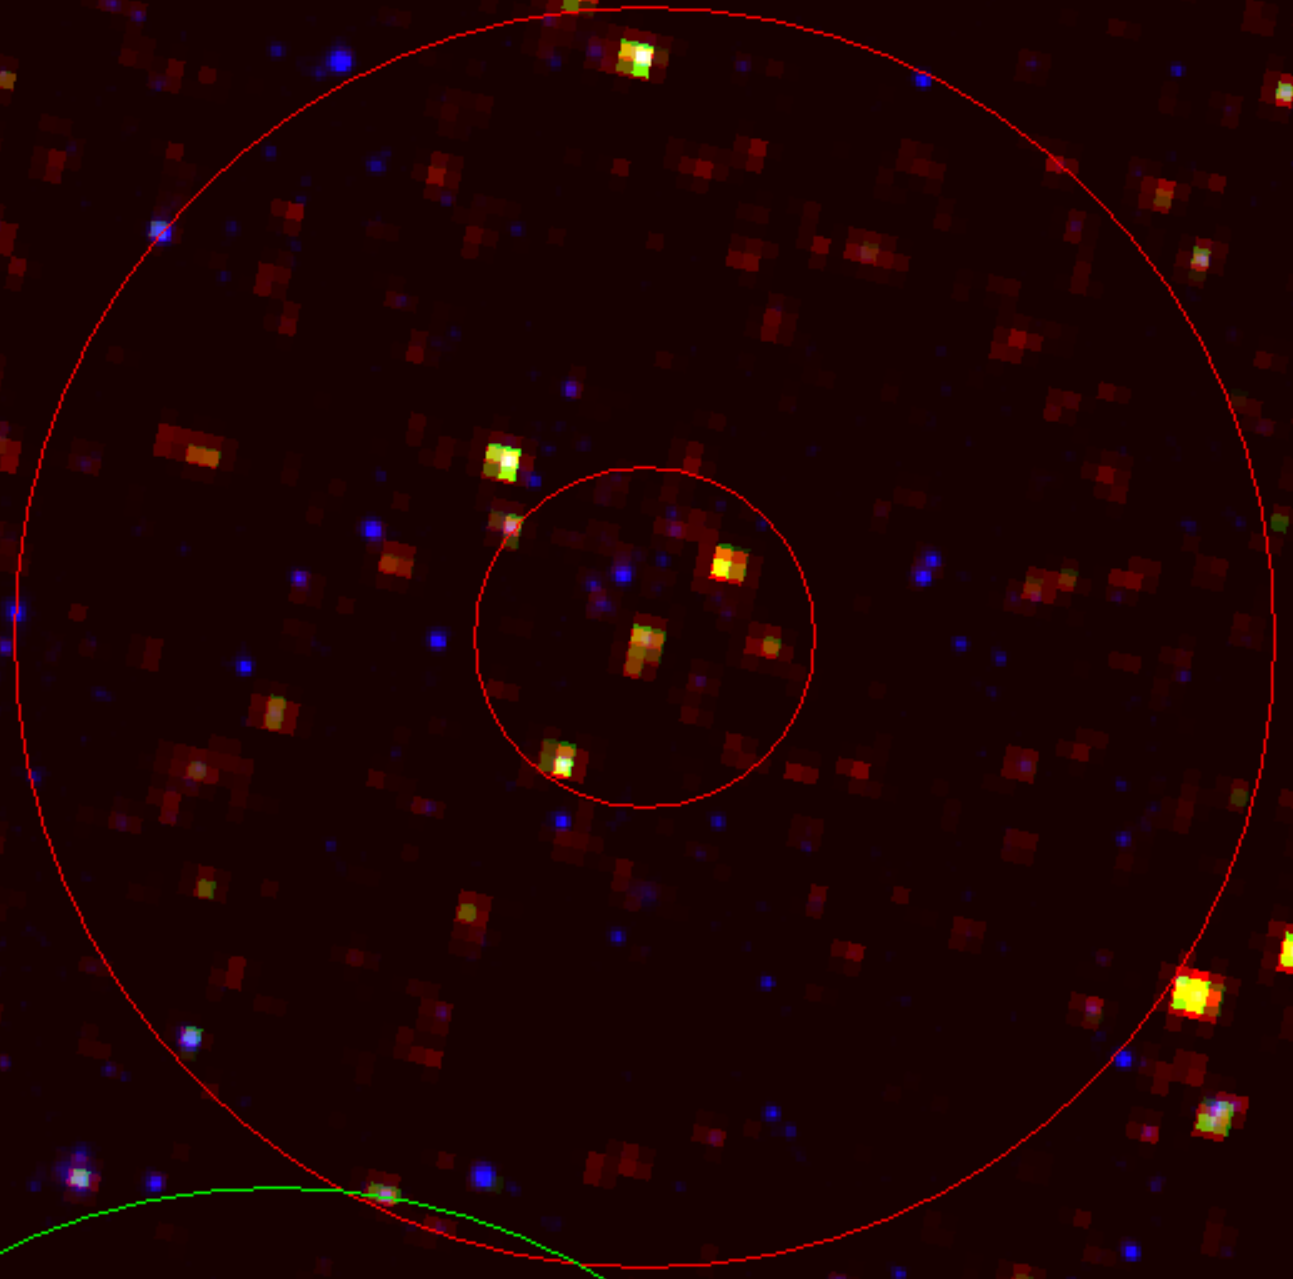}
            \\ RSG 4881 - 27 Myr
        \end{minipage}
        \begin{minipage}{.3\textwidth}
            \centering
            \includegraphics[width=\textwidth]{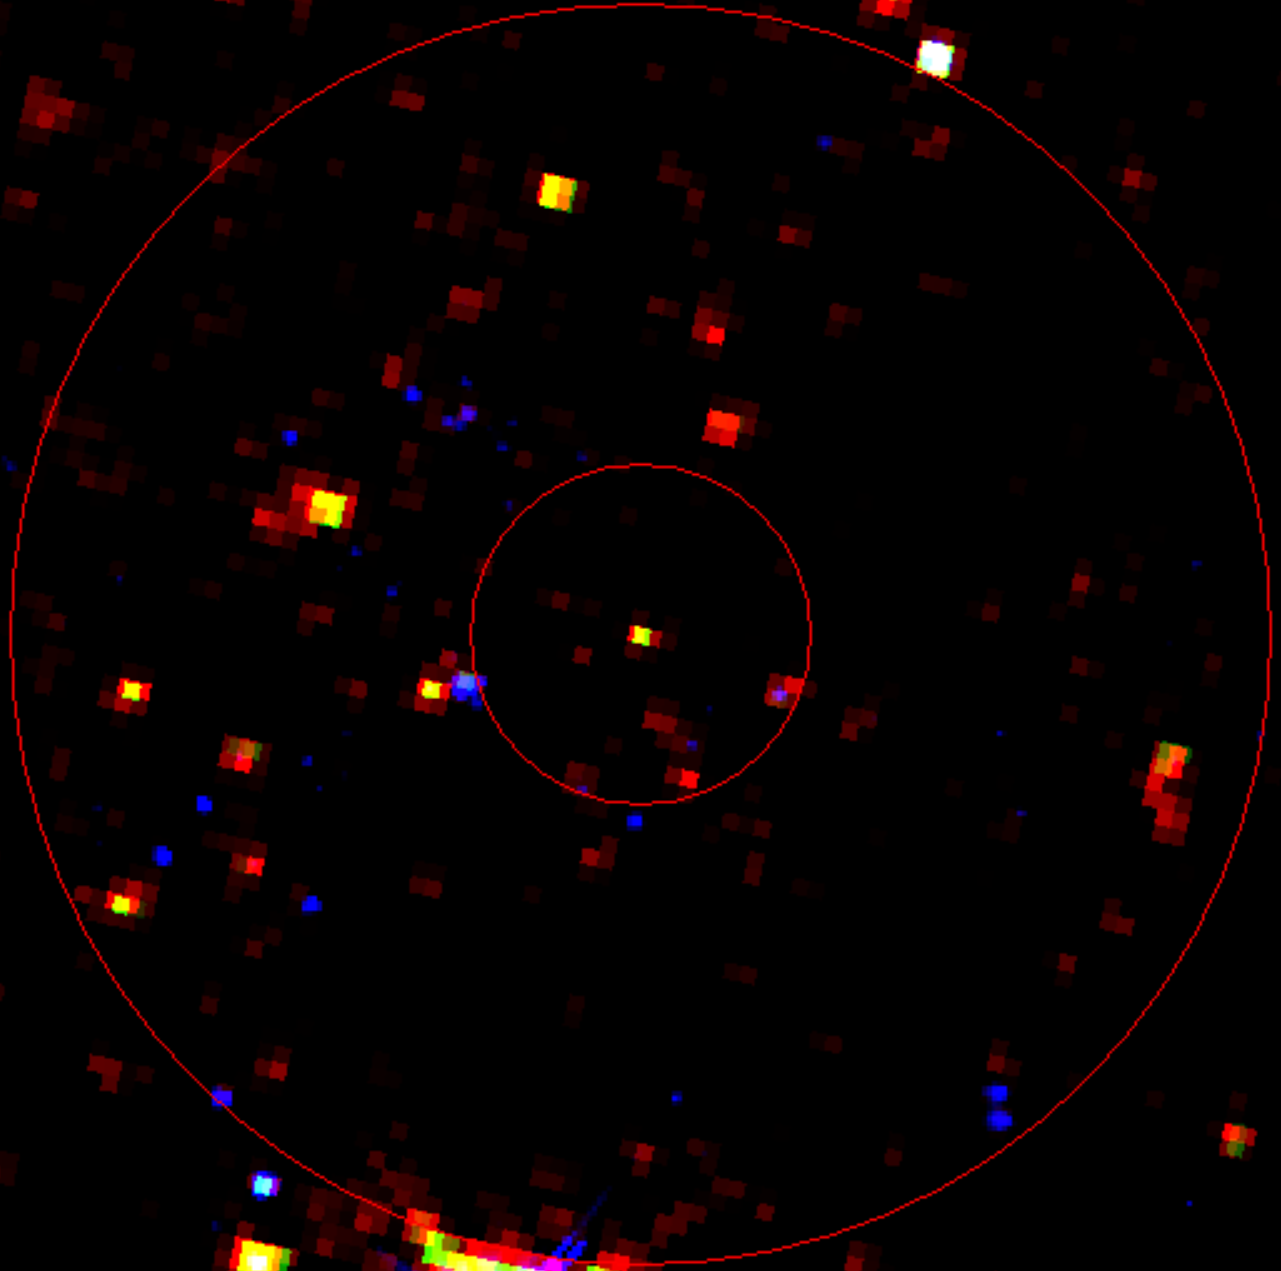}
            \\ RSG 2748 - 21 Myr
        \end{minipage}
        \begin{minipage}{.3\textwidth}
            \centering
            \includegraphics[width=\textwidth]{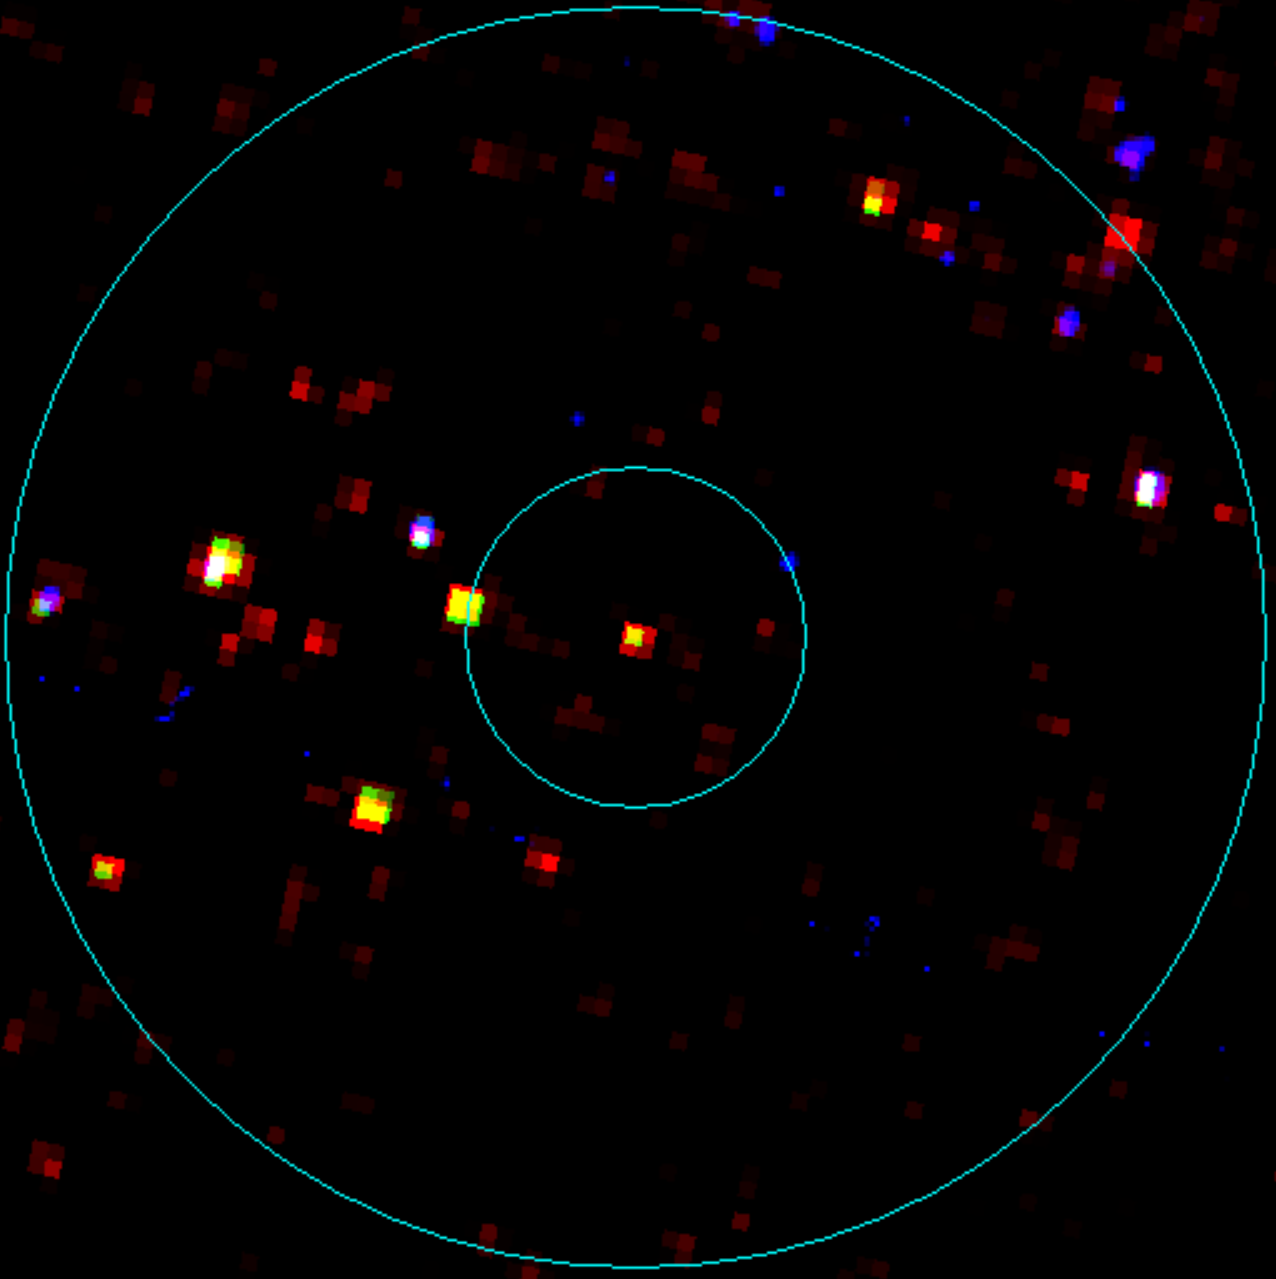}
            \\ RSG 3485 - 9 Myr
        \end{minipage}
        \begin{minipage}{.3\textwidth}
            \centering
            \includegraphics[width=\textwidth]{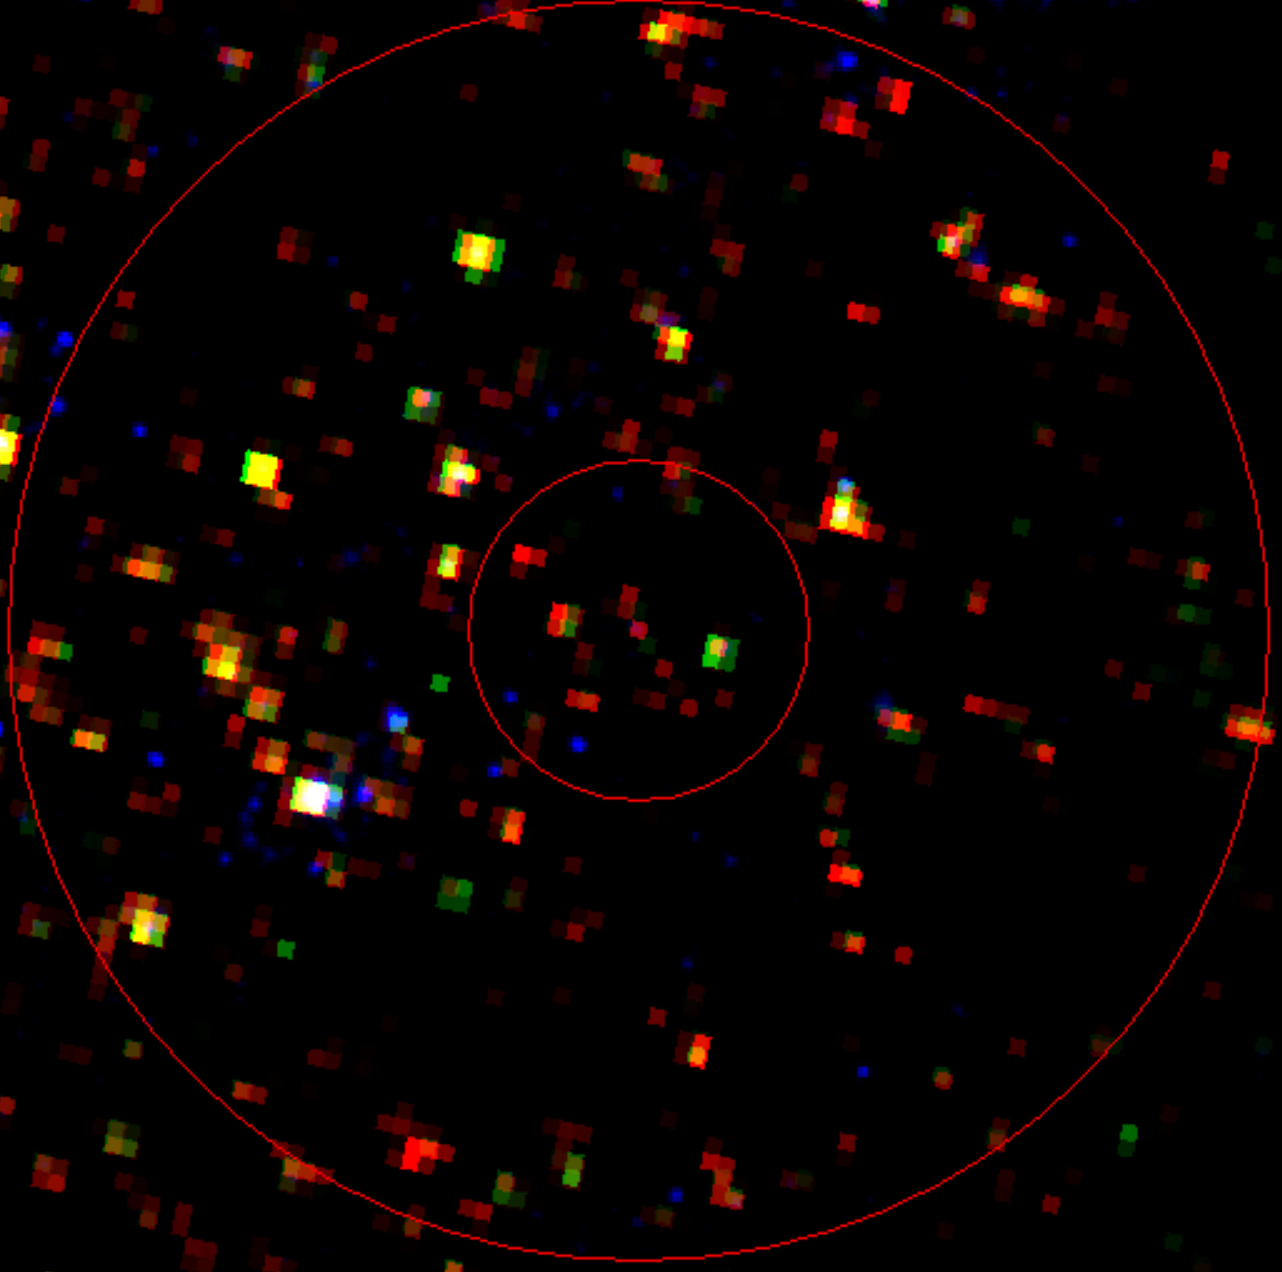}
            \\ RSG 3532 - 29 Myr
        \end{minipage}
        \begin{minipage}{.3\textwidth}
            \centering
            \includegraphics[width=\textwidth]{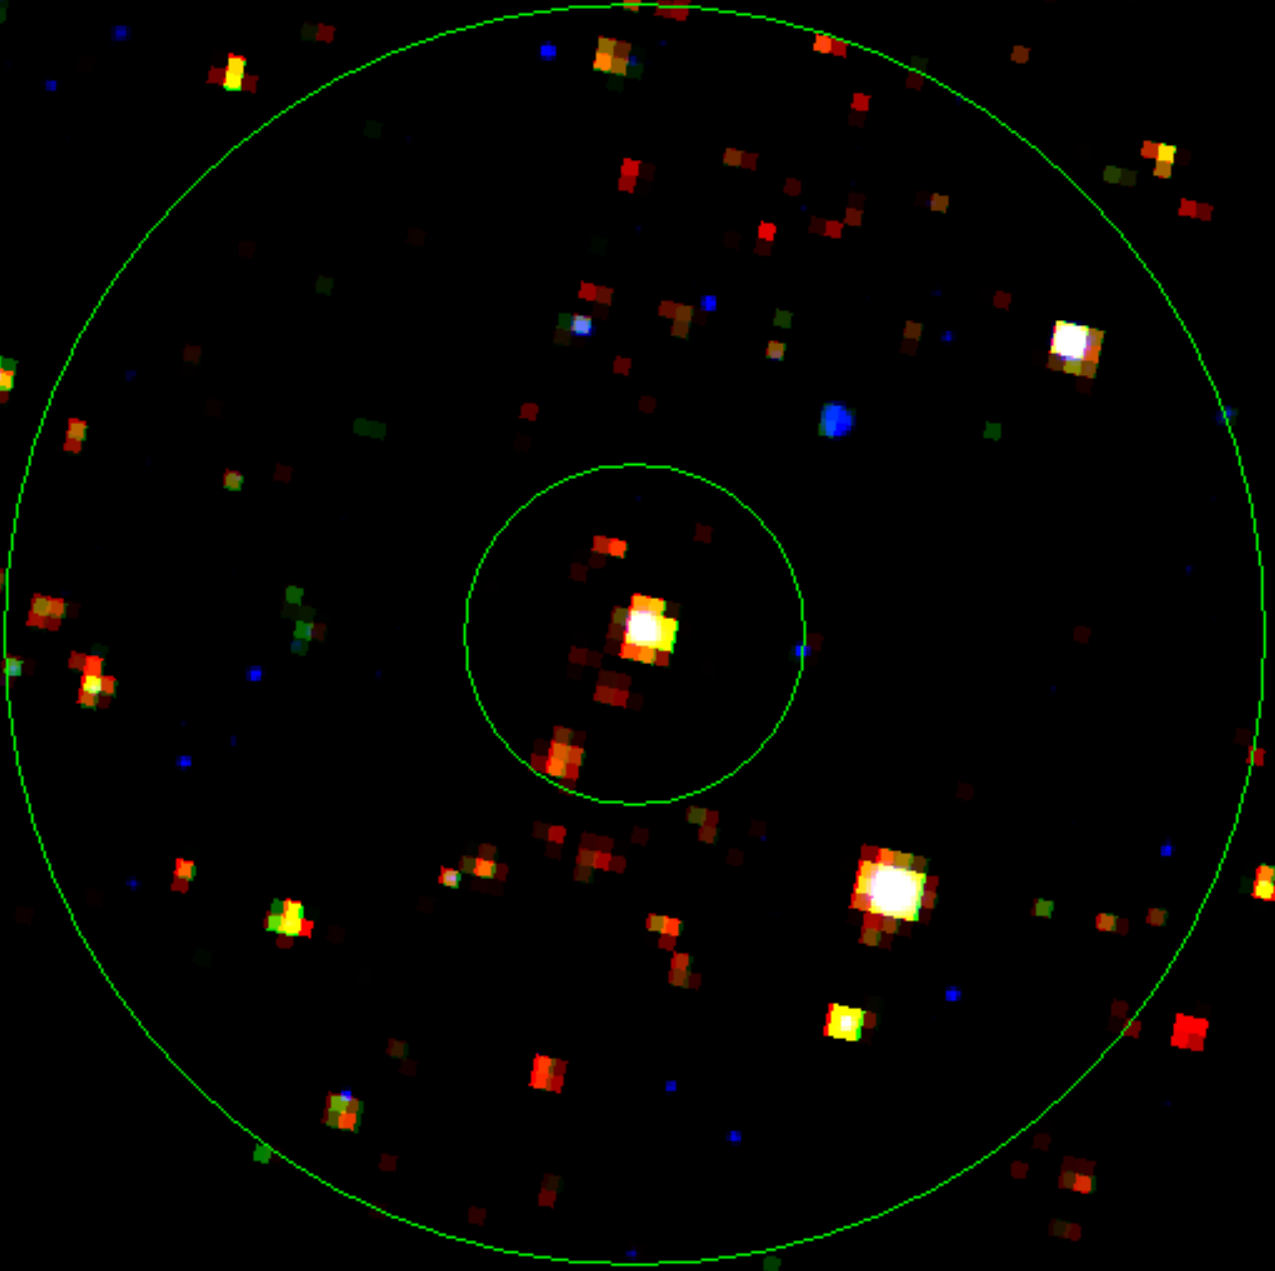}
            \\ RSG 3059 - 15 Myr
        \end{minipage}
        \begin{minipage}{.3\textwidth}
            \centering
            \includegraphics[width=\textwidth]{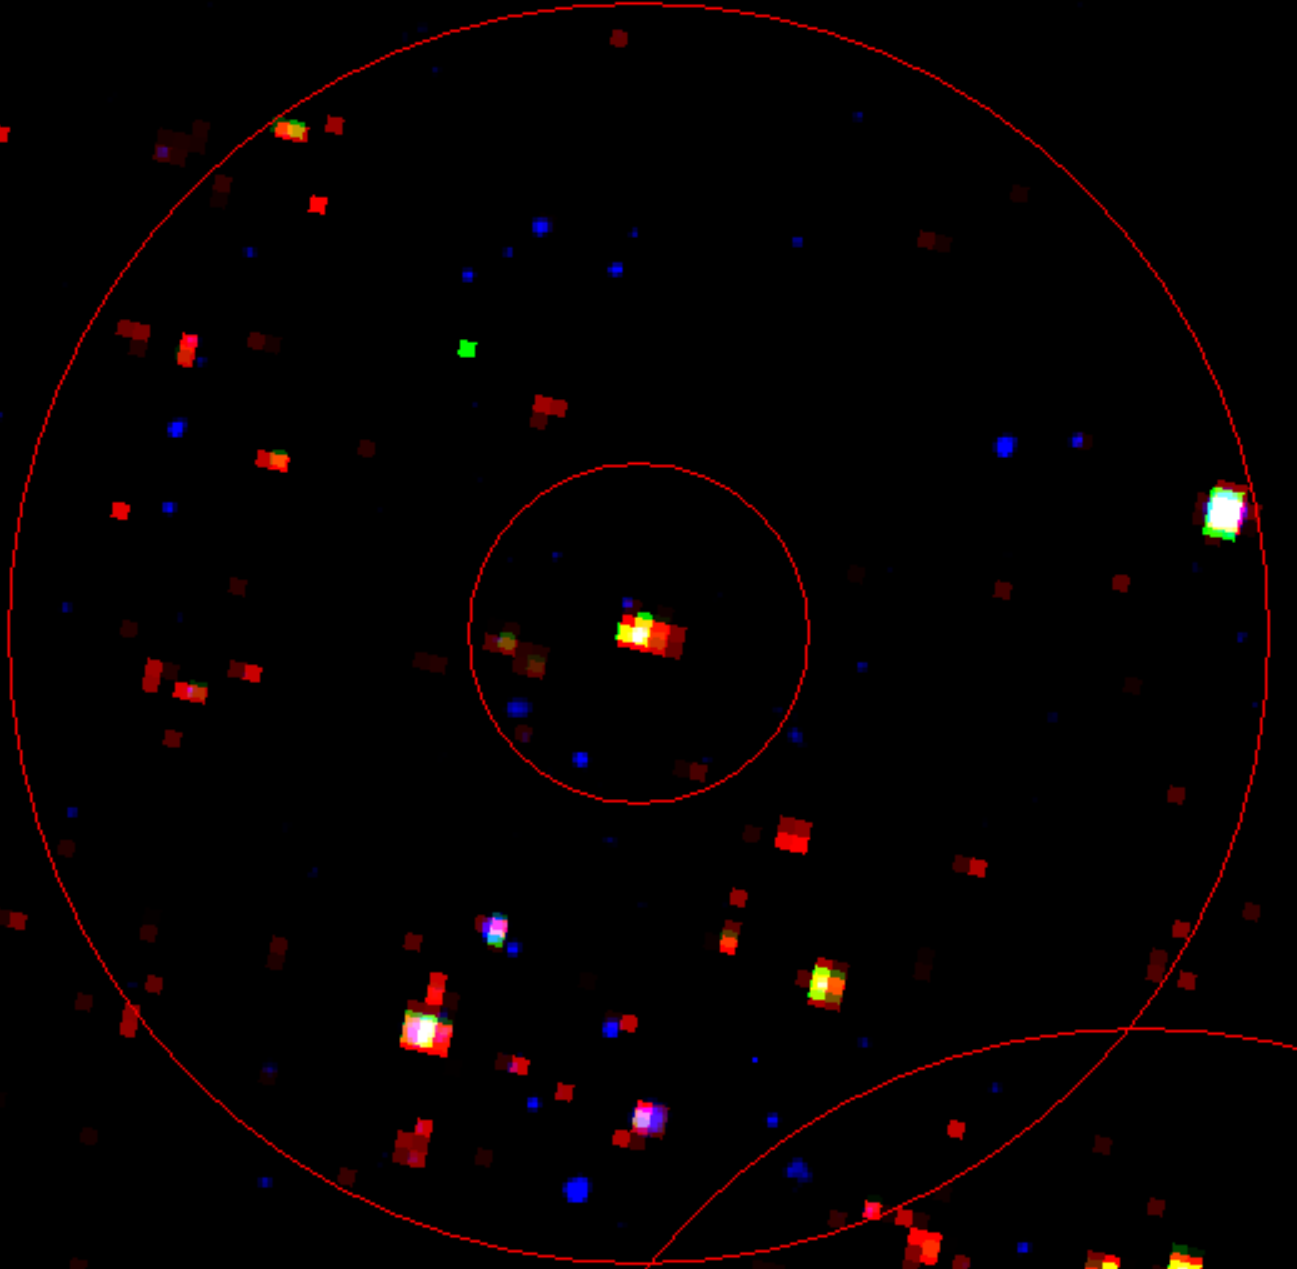}
            \\ RSG 5026 - 29 Myr
        \end{minipage}
        \begin{minipage}{.3\textwidth}
            \centering
            \includegraphics[width=\textwidth]{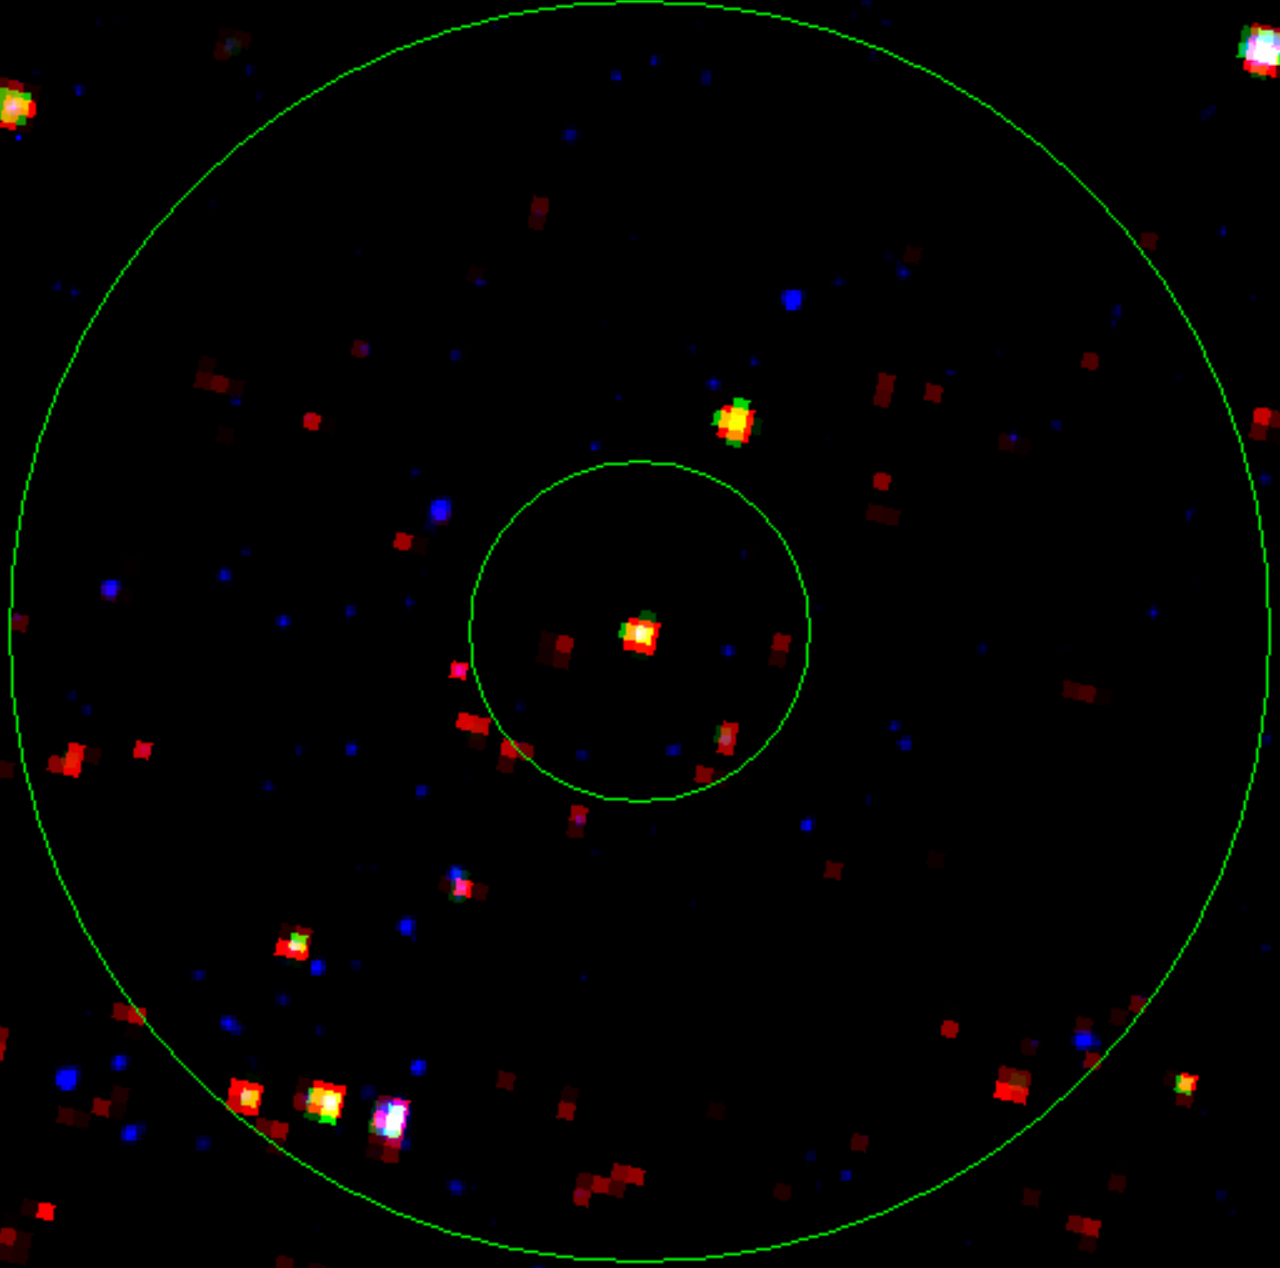}
            \\ RSG 4906 - 11 Myr
        \end{minipage}
    \end{figure}

    \begin{figure}[hbt!]
        \centering
        \begin{minipage}{.3\textwidth}
            \centering
            \includegraphics[width=\textwidth]{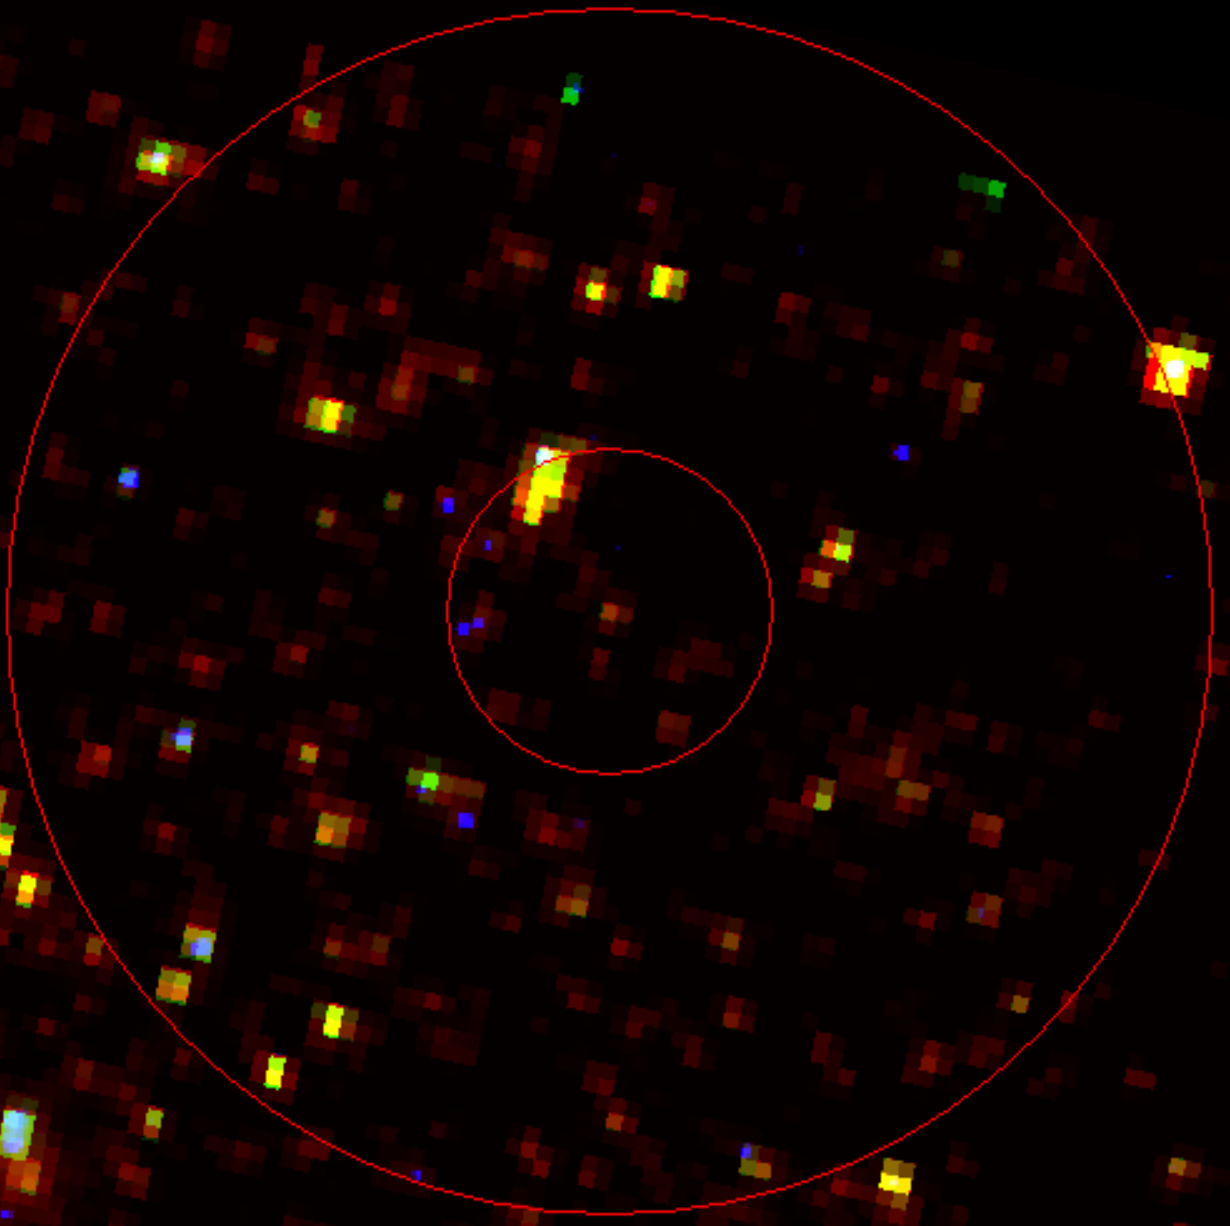}
            \\ RSG 2214 - 27 Myr
        \end{minipage}
        \begin{minipage}{.3\textwidth}
            \centering
            \includegraphics[width=\textwidth]{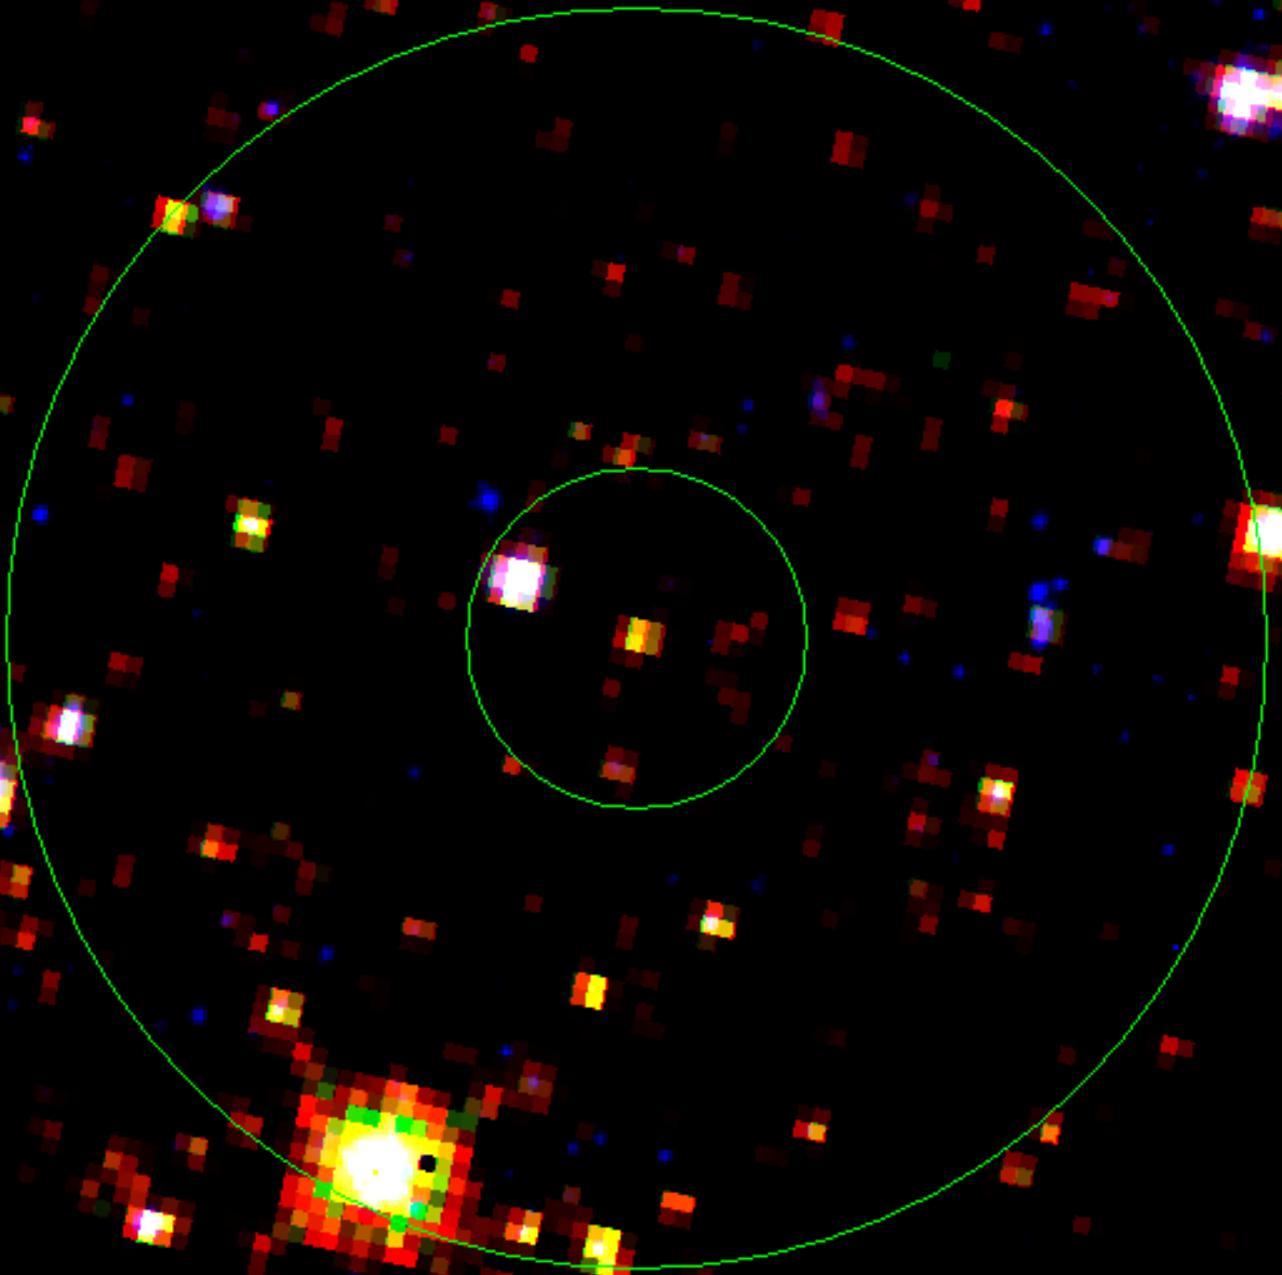}
            \\ RSG 6822 - 12 Myr
        \end{minipage}
        \begin{minipage}{.3\textwidth}
            \centering
            \includegraphics[width=\textwidth]{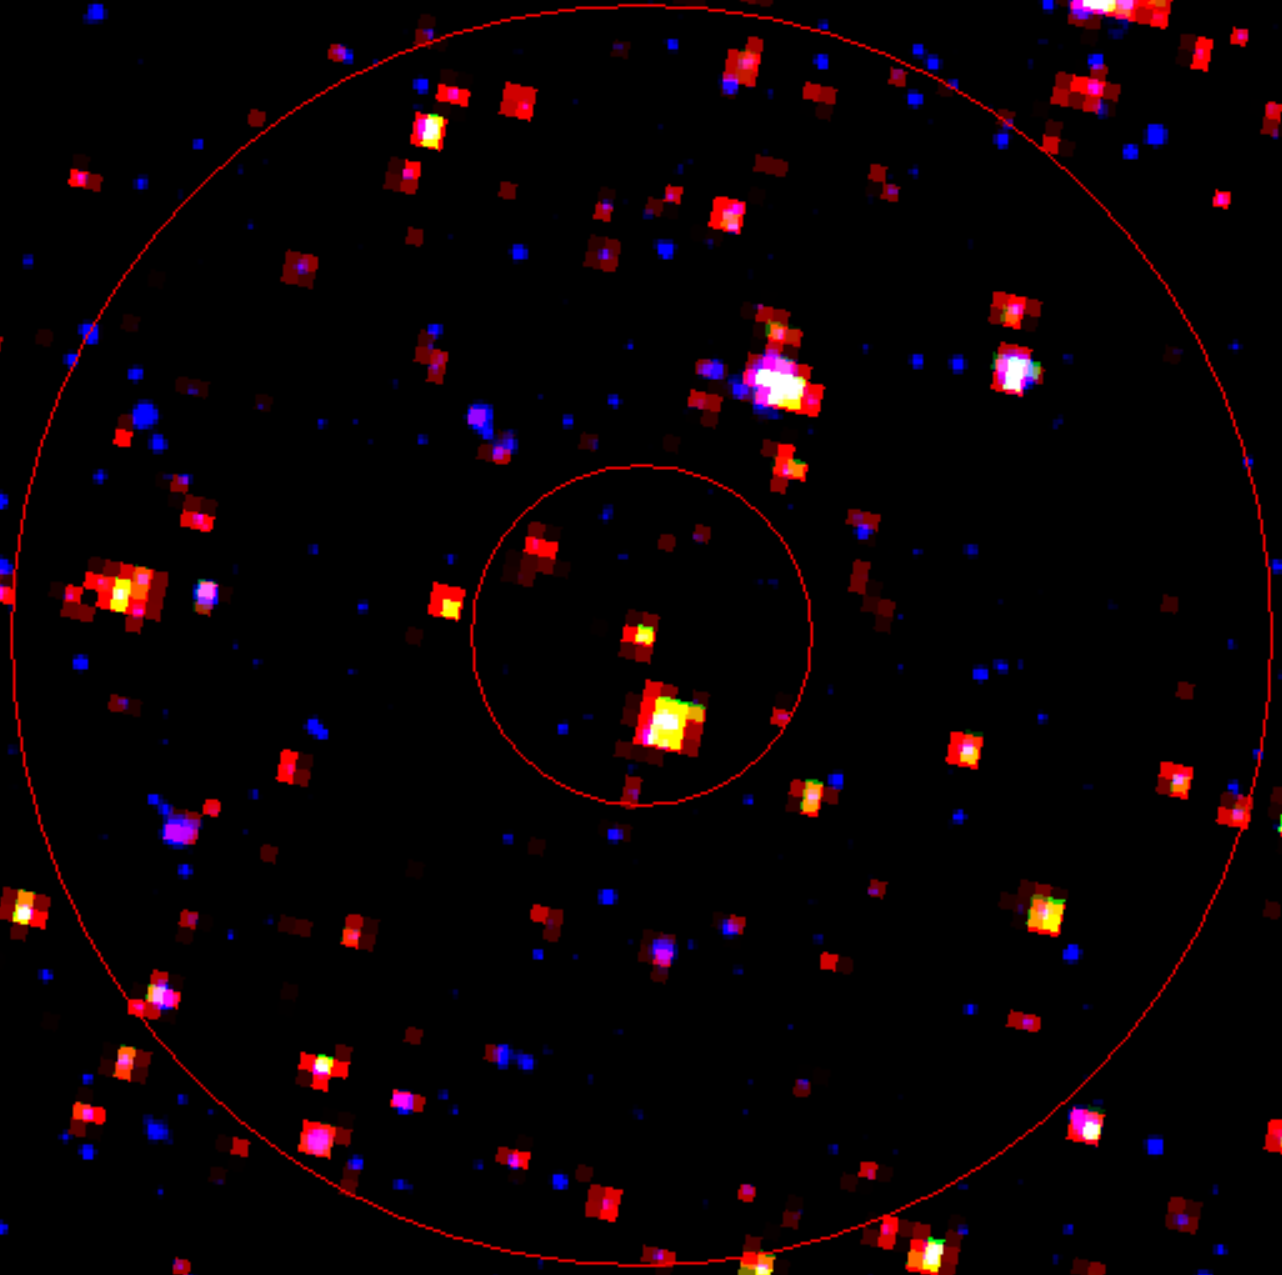}
            \\ RSG 3336 - 24 Myr
        \end{minipage}
        \begin{minipage}{.3\textwidth}
            \centering
            \includegraphics[width=\textwidth]{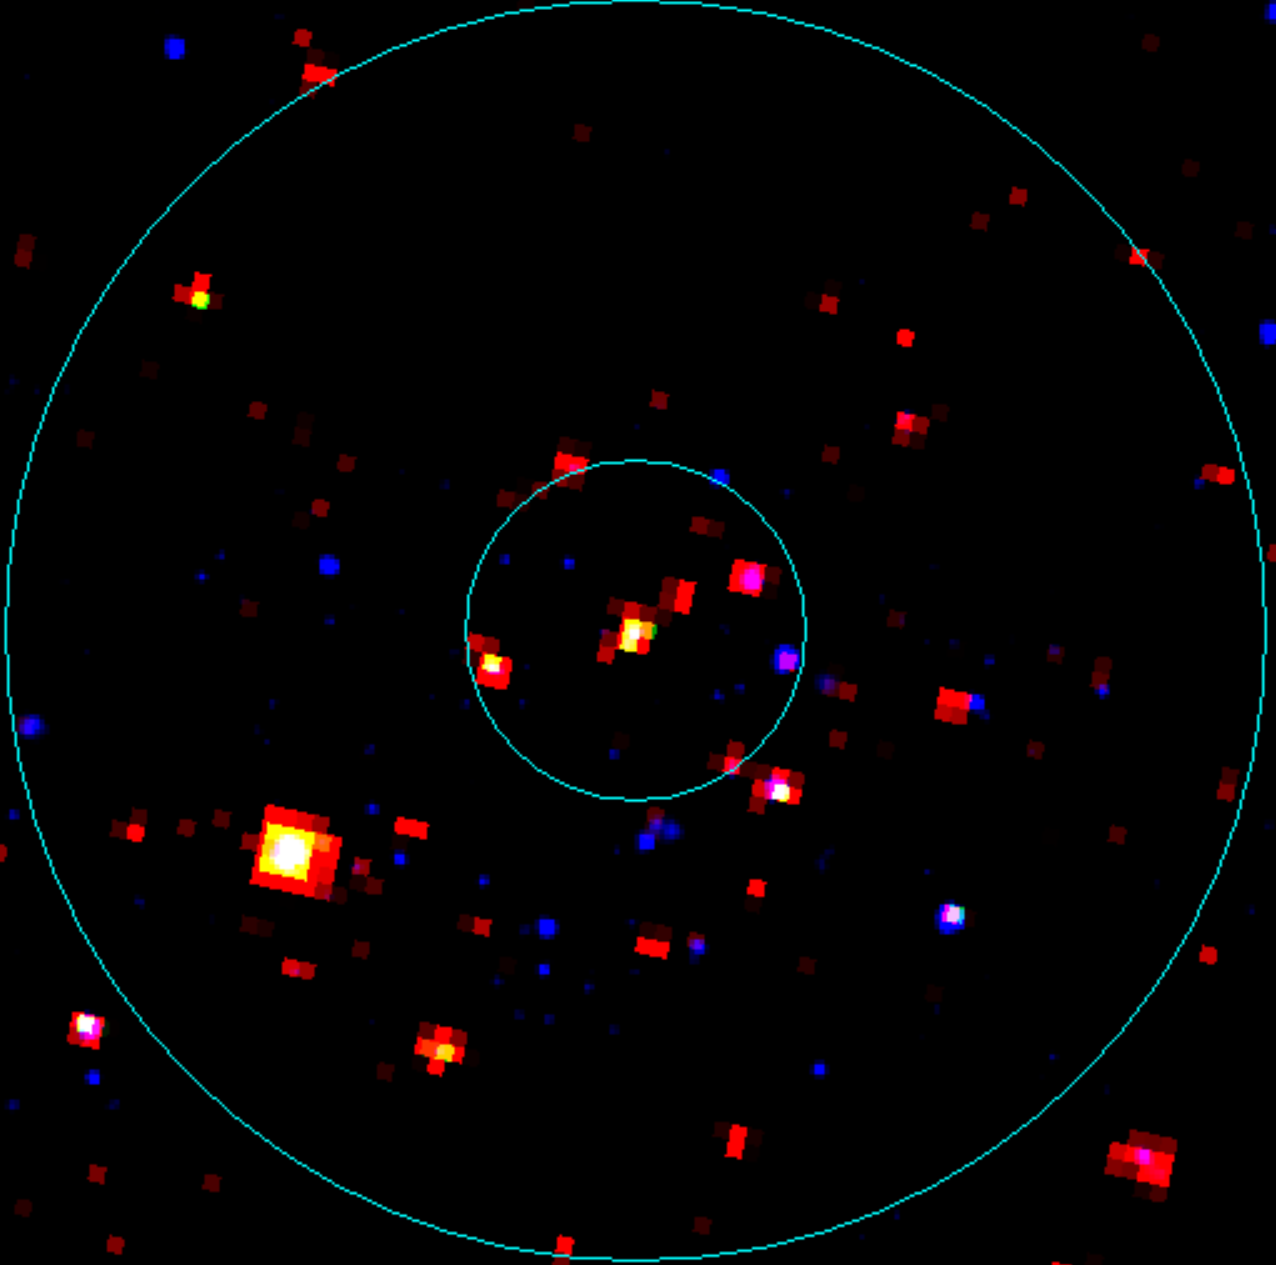}
            \\ RSG 3091 - 7 Myr
        \end{minipage}
        \begin{minipage}{.3\textwidth}
            \centering
            \includegraphics[width=\textwidth]{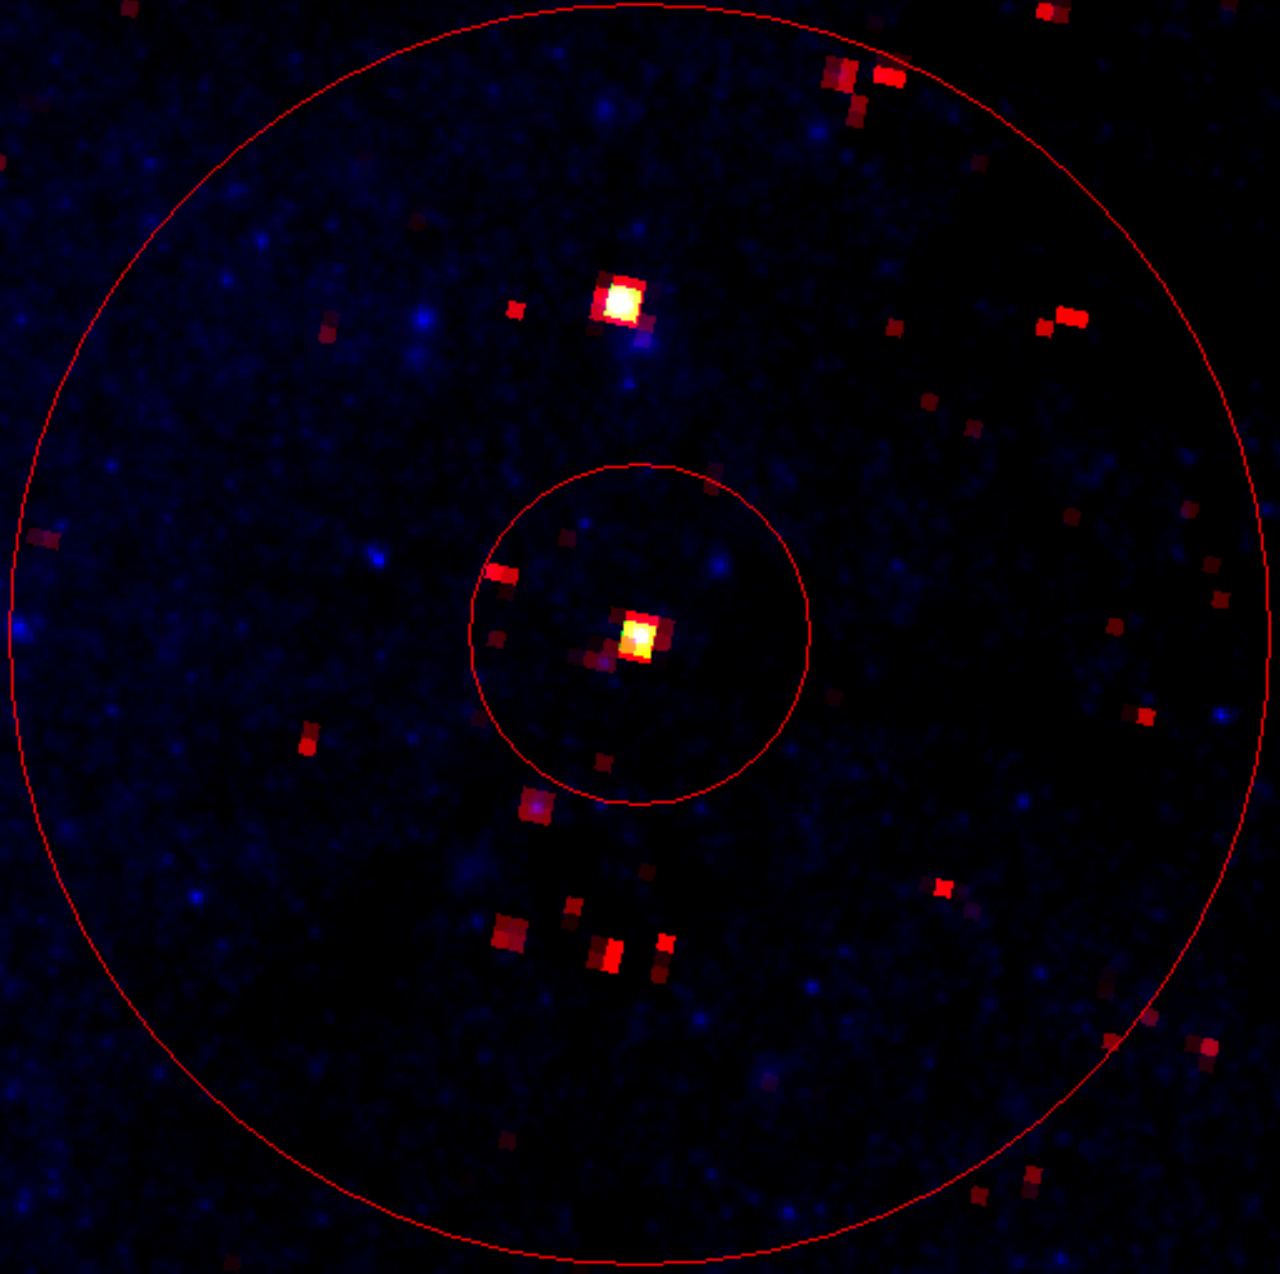}
            \\ RSG 4118 - 29 Myr
        \end{minipage}
        \begin{minipage}{.3\textwidth}
            \centering
            \includegraphics[width=\textwidth]{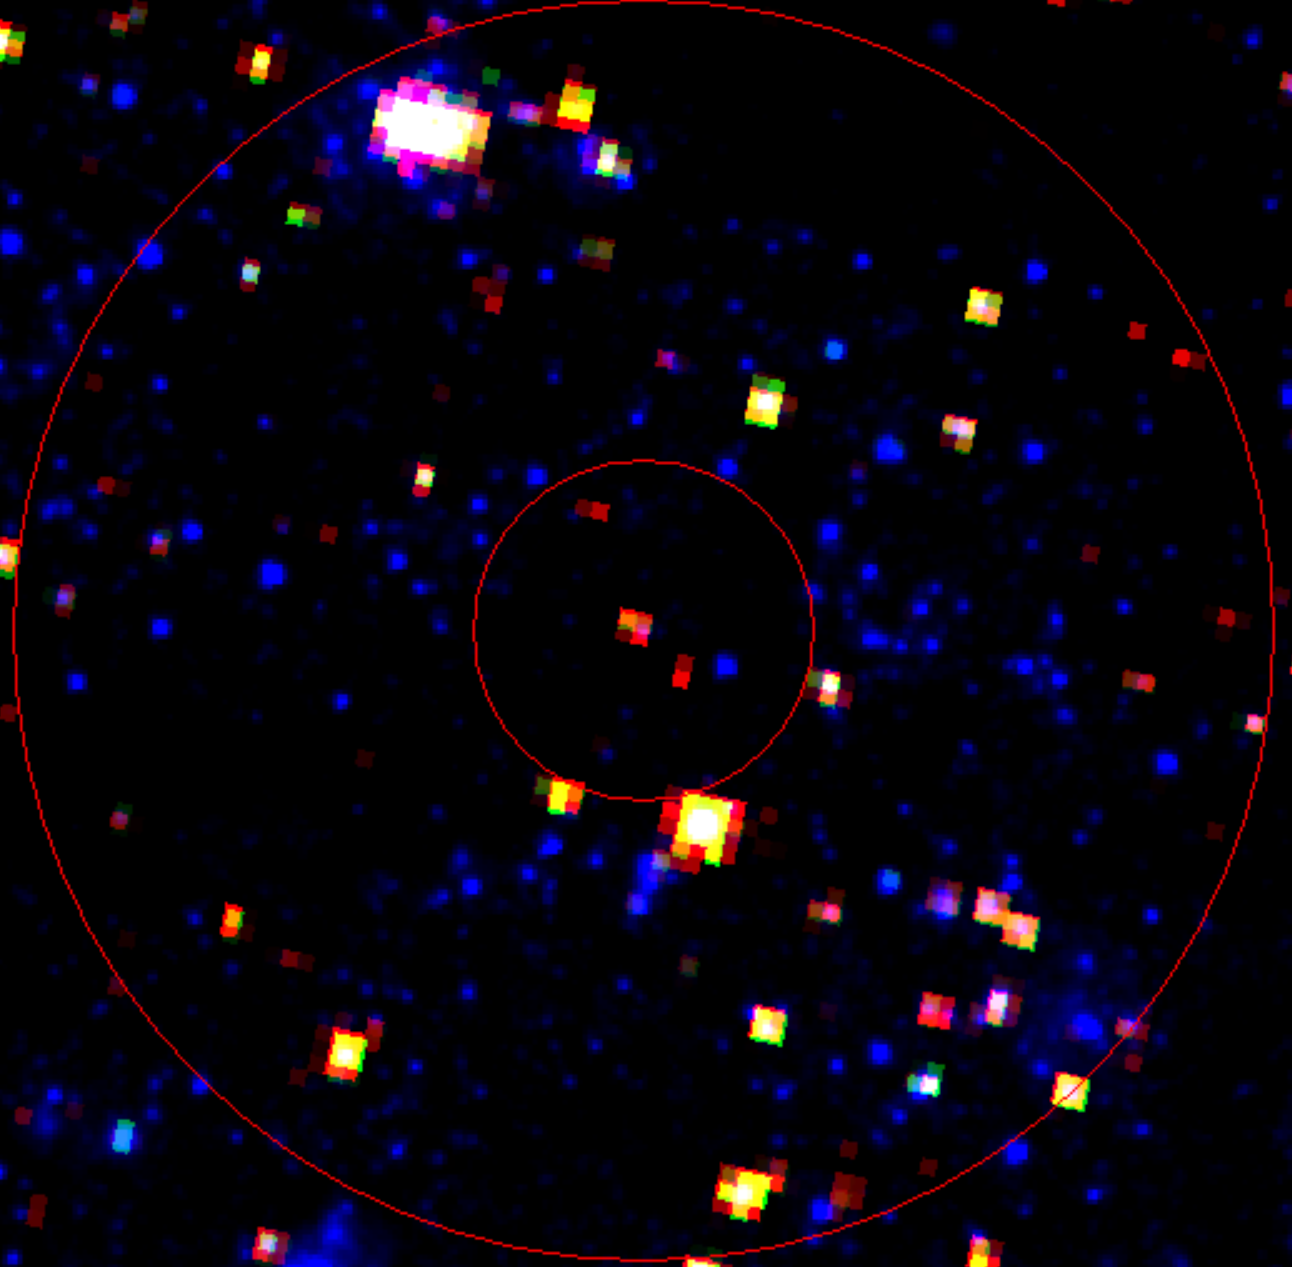}
            \\ RSG 4480 - 27 Myr
        \end{minipage}
        \begin{minipage}{.3\textwidth}
            \centering
            \includegraphics[width=\textwidth]{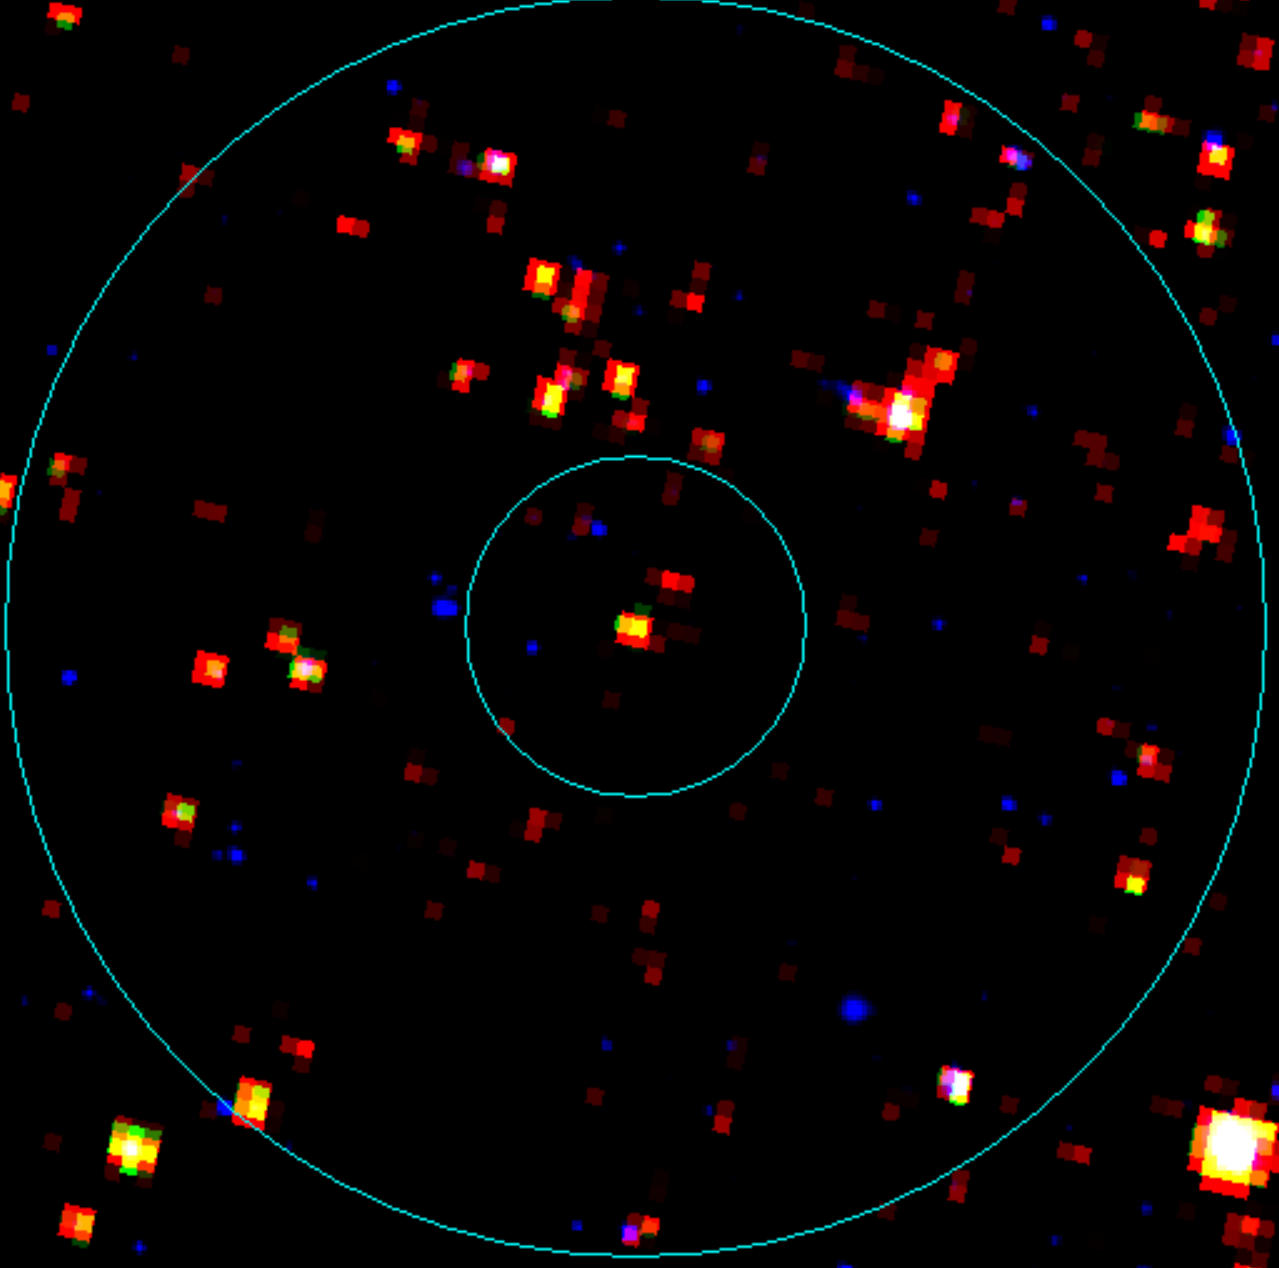}
            \\ RSG 4949 - 9 Myr
        \end{minipage}
        \begin{minipage}{.3\textwidth}
            \centering
            \includegraphics[width=\textwidth]{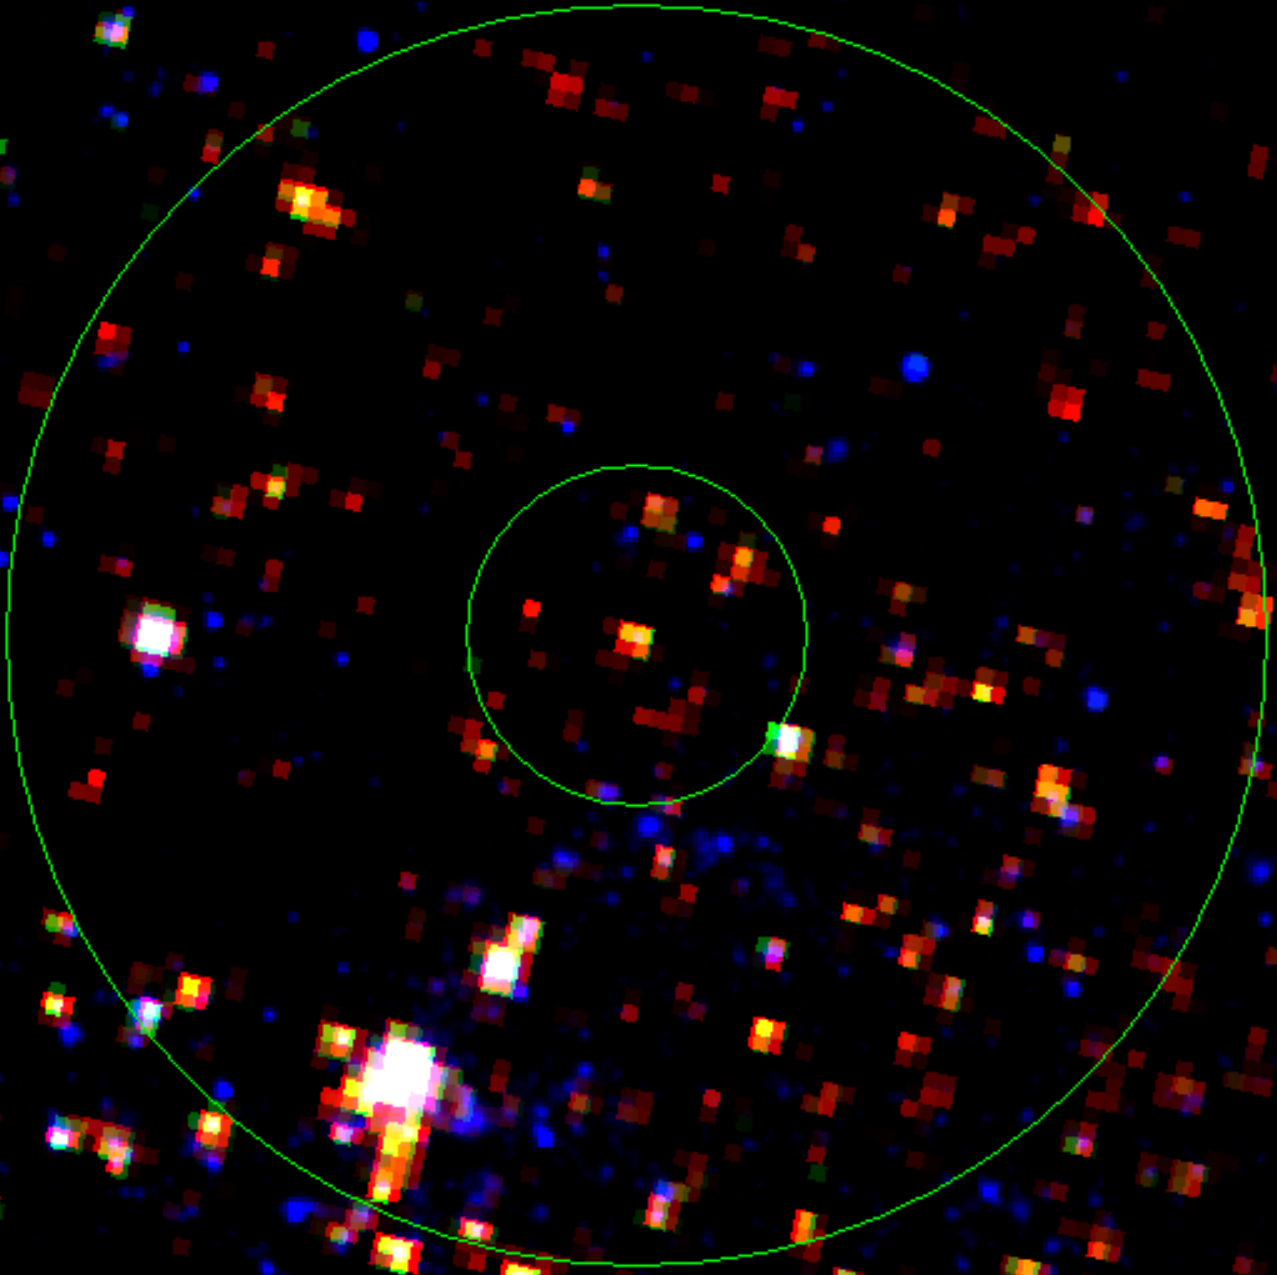}
            \\ RSG 3954 - 11 Myr
        \end{minipage}
        \begin{minipage}{.3\textwidth}
            \centering
            \includegraphics[width=\textwidth]{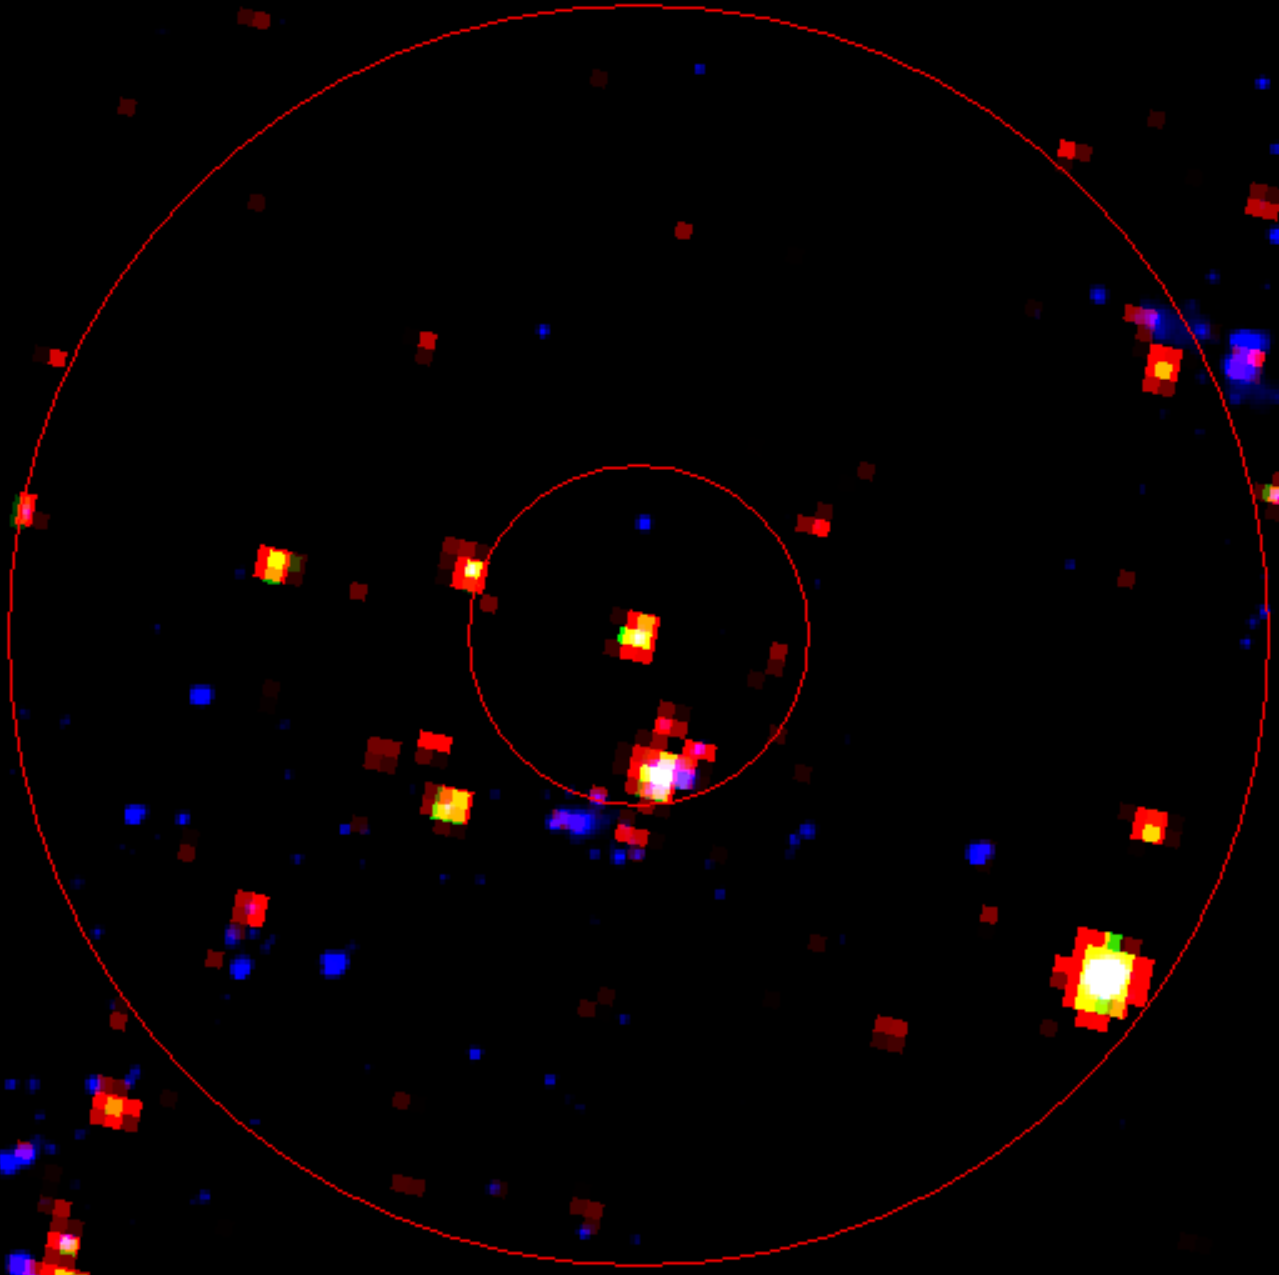}
            \\ RSG 2813 - 27 Myr
        \end{minipage}
        \begin{minipage}{.3\textwidth}
            \centering
            \includegraphics[width=\textwidth]{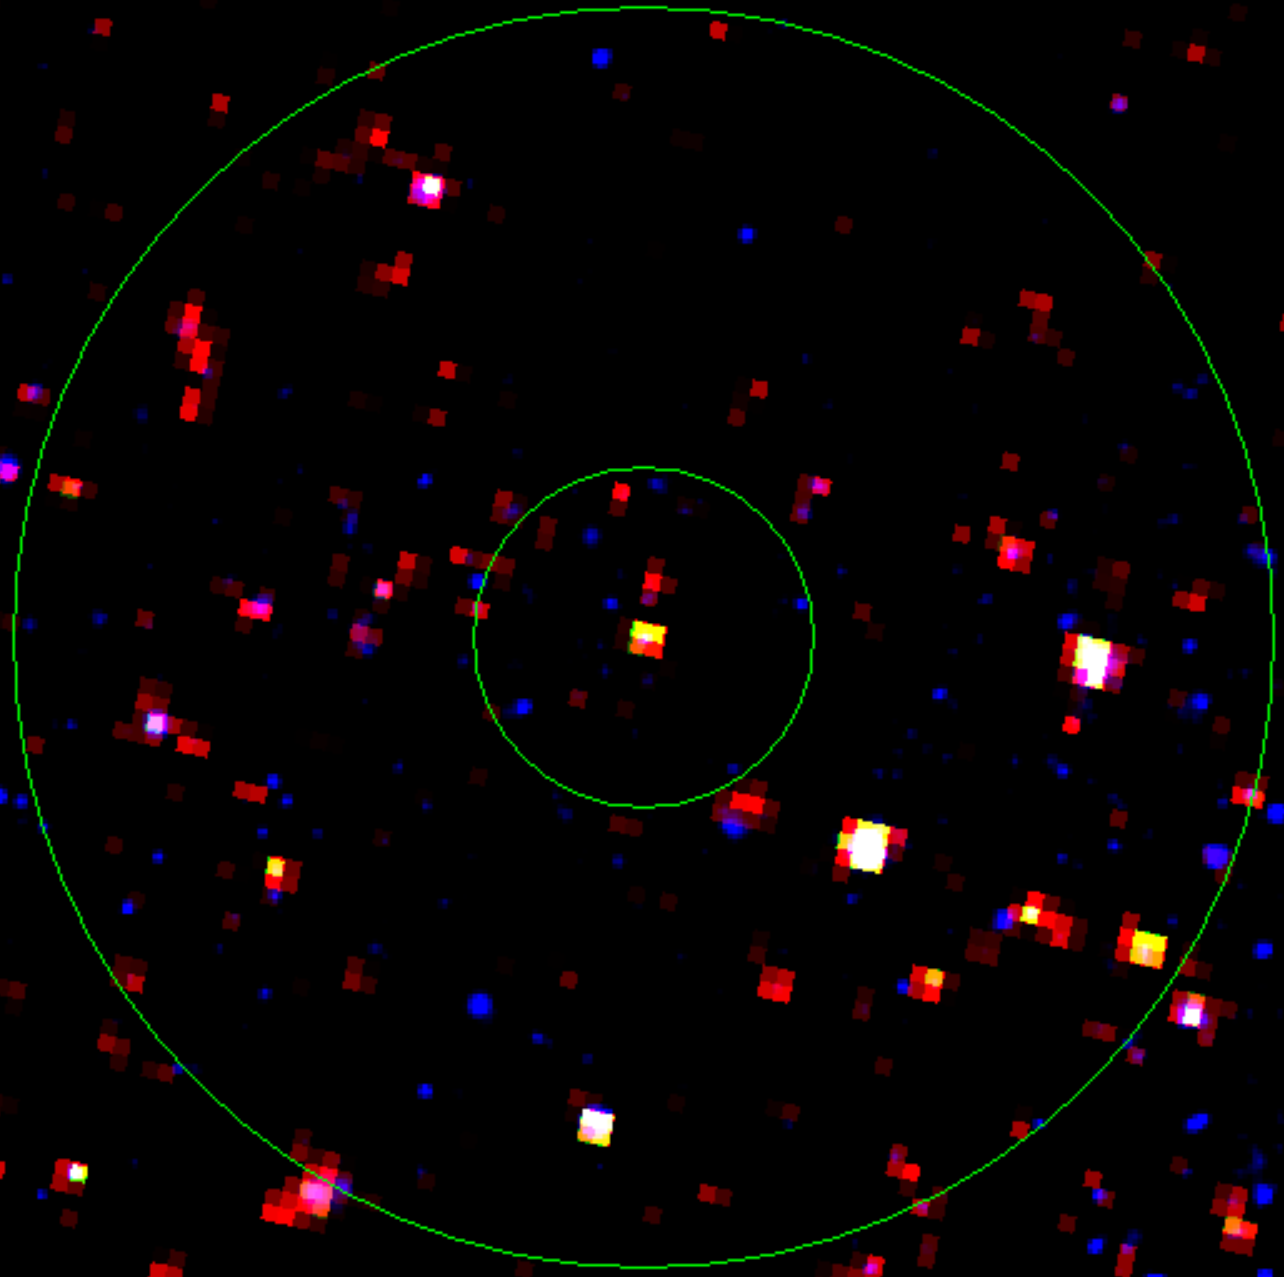}
            \\ RSG 3561 - 17 Myr
        \end{minipage}
        \begin{minipage}{.3\textwidth}
            \centering
            \includegraphics[width=\textwidth]{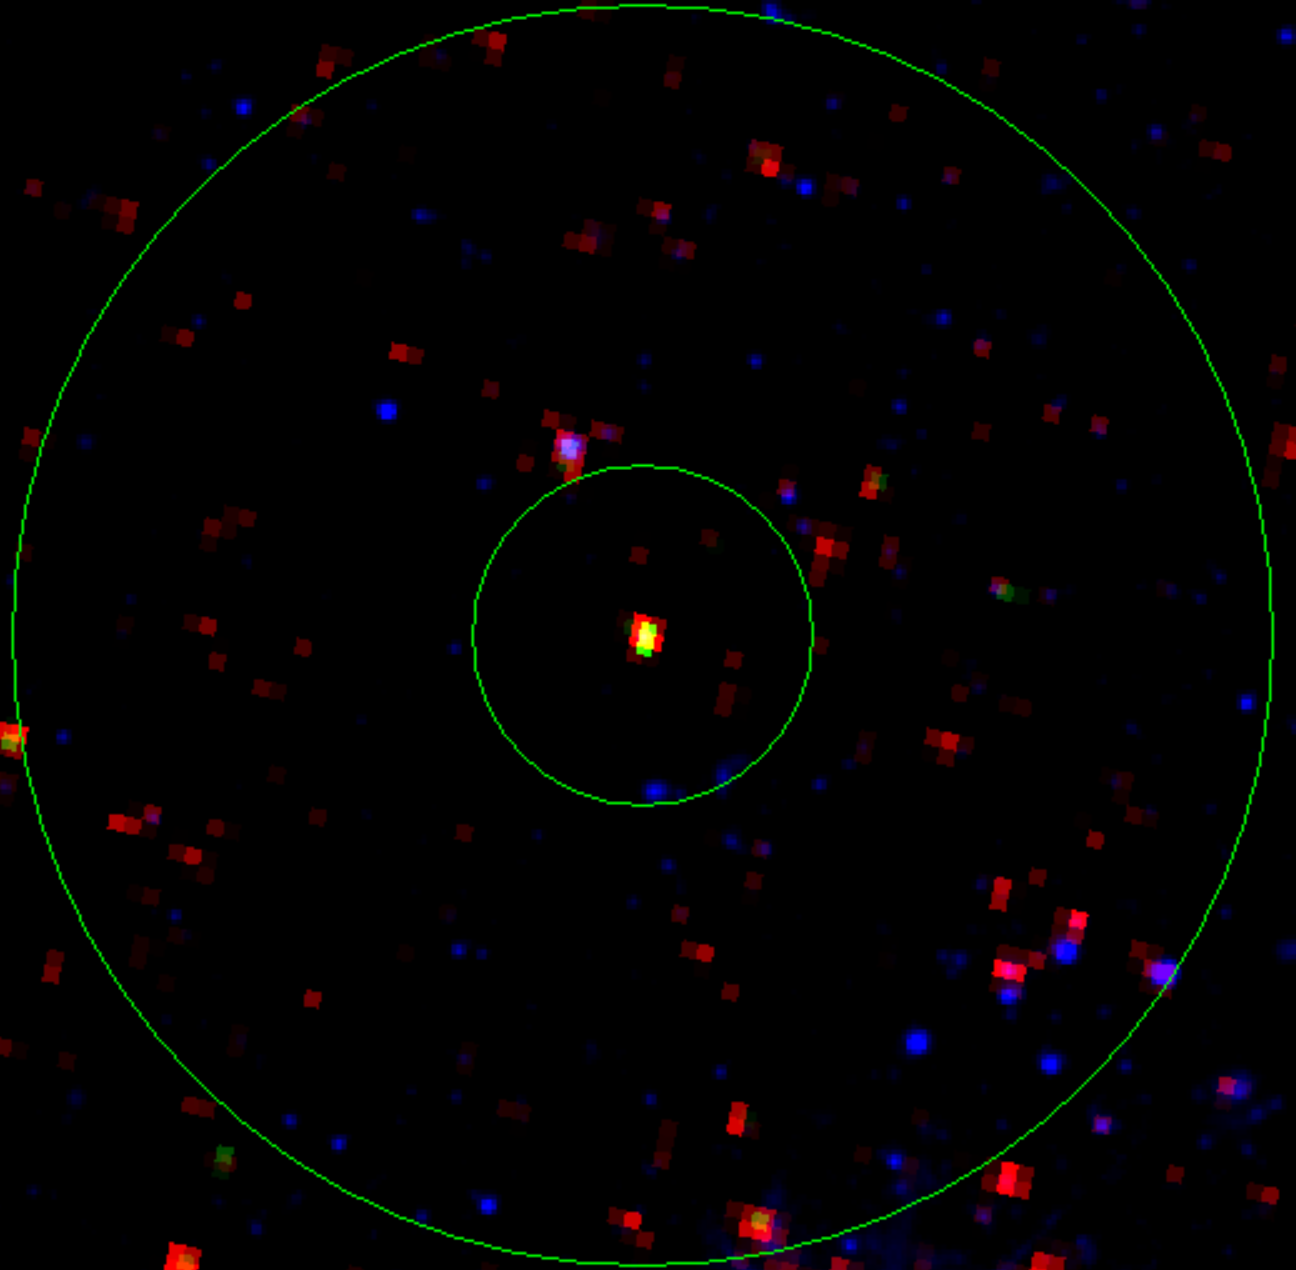}
            \\ RSG 6318 - 19 Myr
        \end{minipage}
        \begin{minipage}{.3\textwidth}
            \centering
            \includegraphics[width=\textwidth]{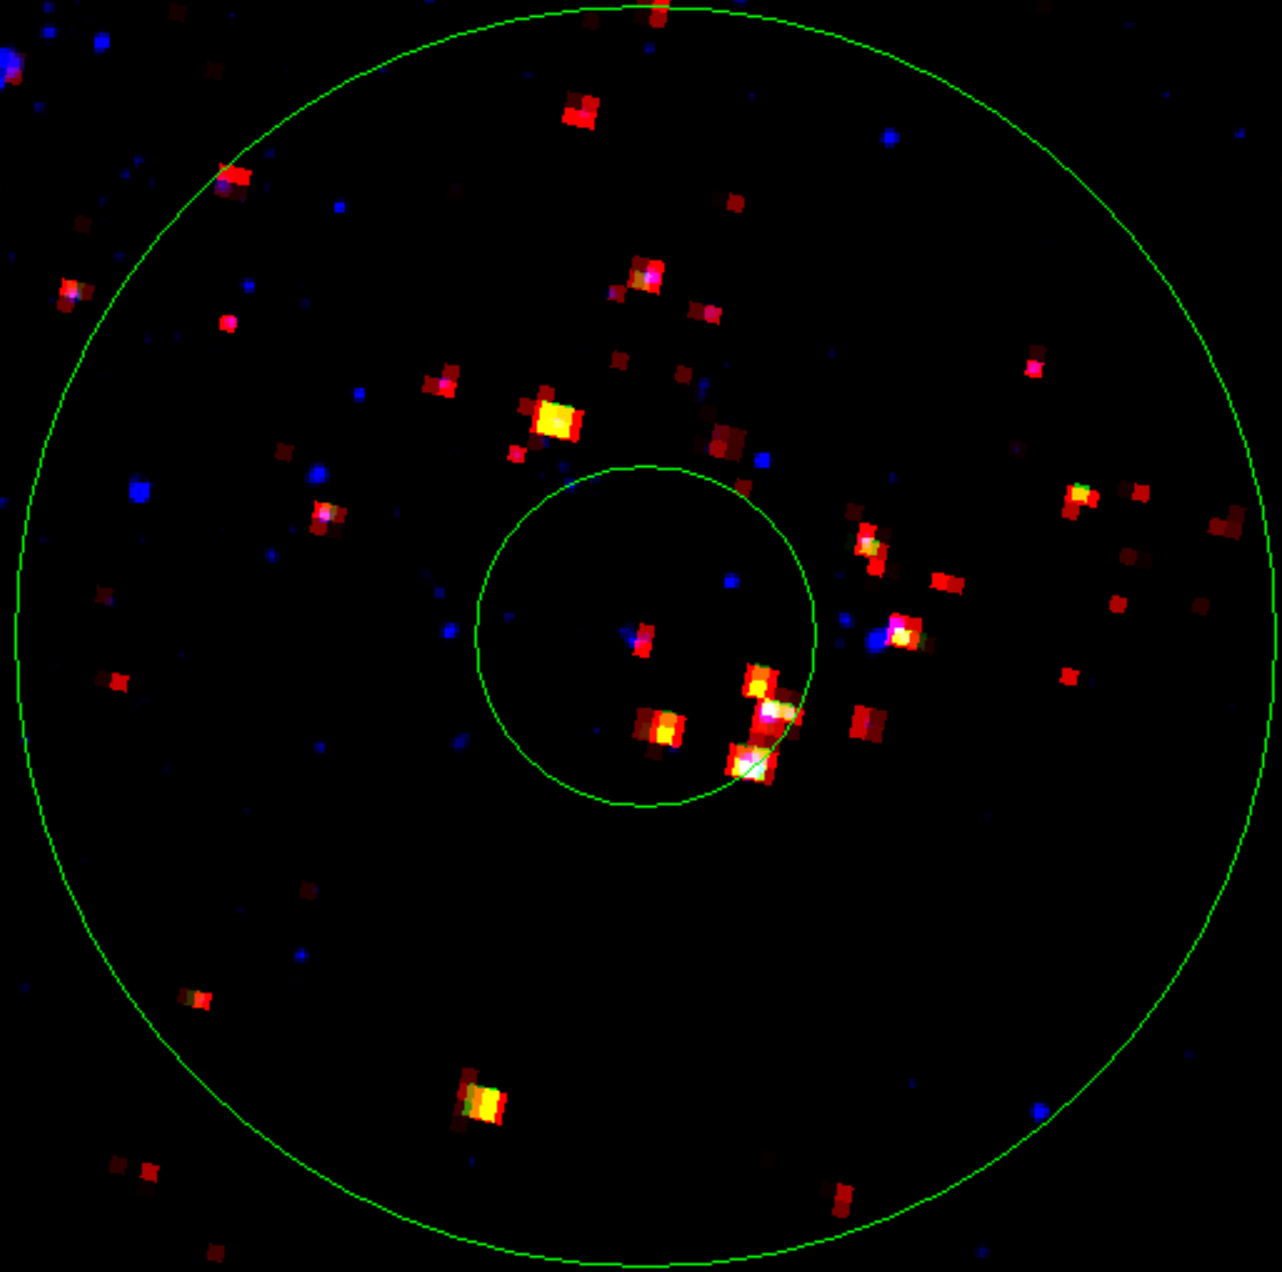}
            \\ RSG 2171 - 17 Myr
        \end{minipage}
    \end{figure}

    \begin{figure}[hbt!]
        \centering
        \begin{minipage}{.3\textwidth}
            \centering
            \includegraphics[width=\textwidth]{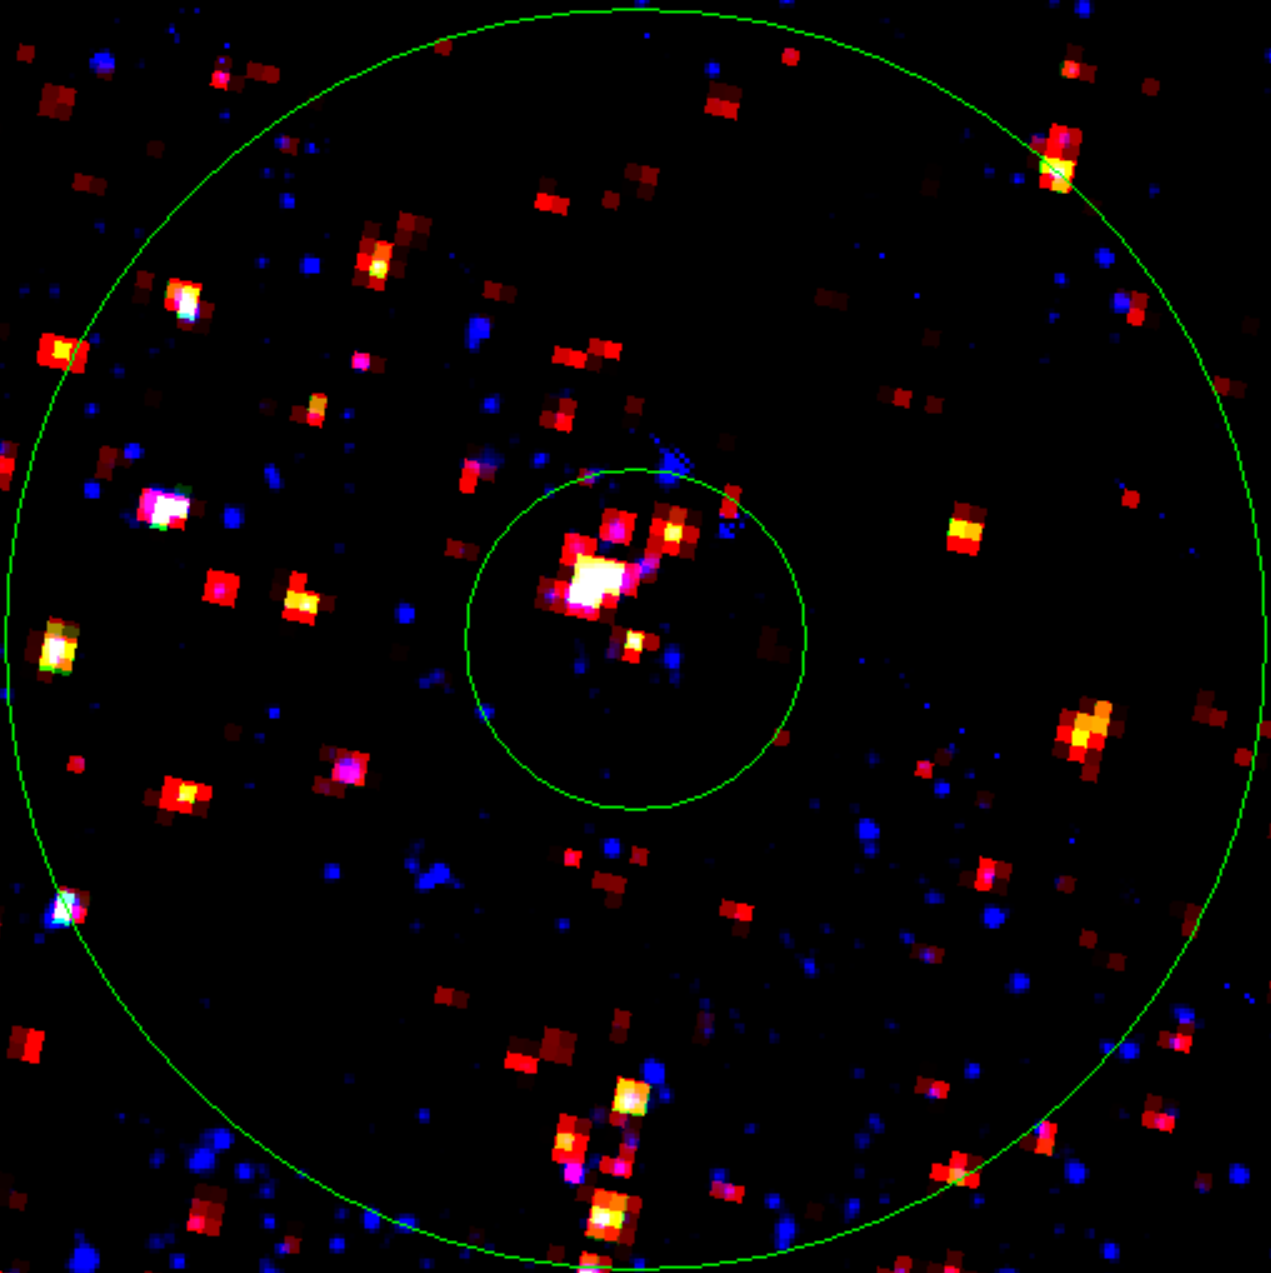}
            \\ RSG 2424 - 15 Myr
        \end{minipage}
        \begin{minipage}{.3\textwidth}
            \centering
            \includegraphics[width=\textwidth]{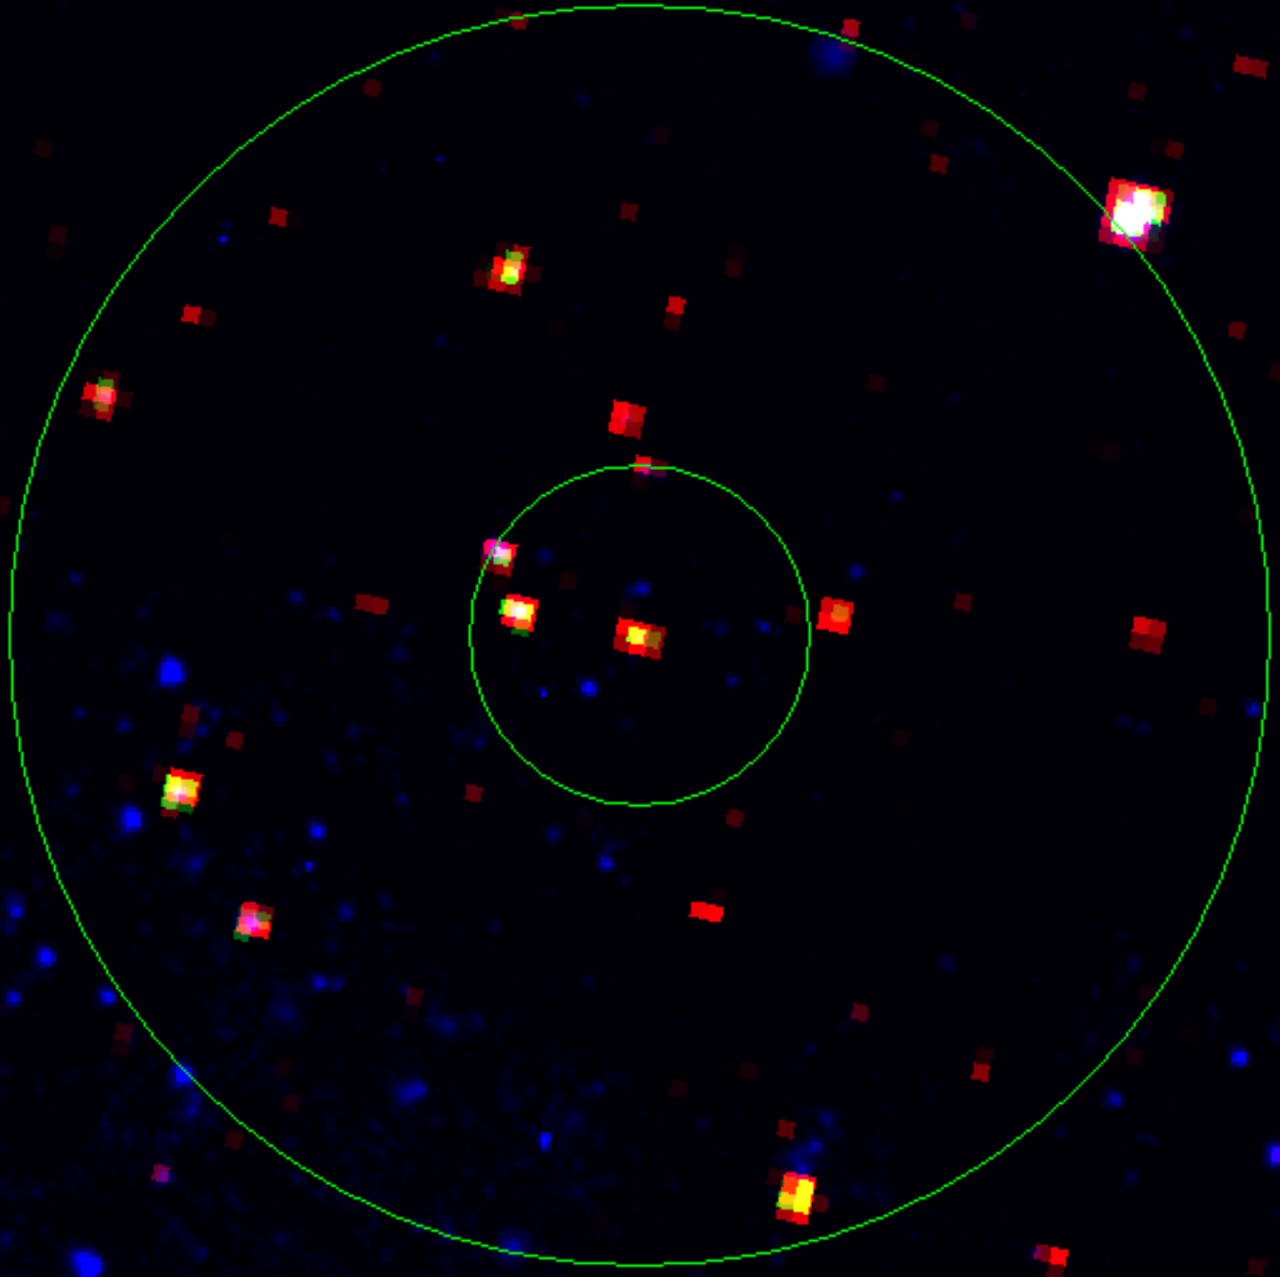}
            \\ RSG 4972 - 17 Myr
        \end{minipage}
            \begin{minipage}{.3\textwidth}
            \centering
            \includegraphics[width=\textwidth]{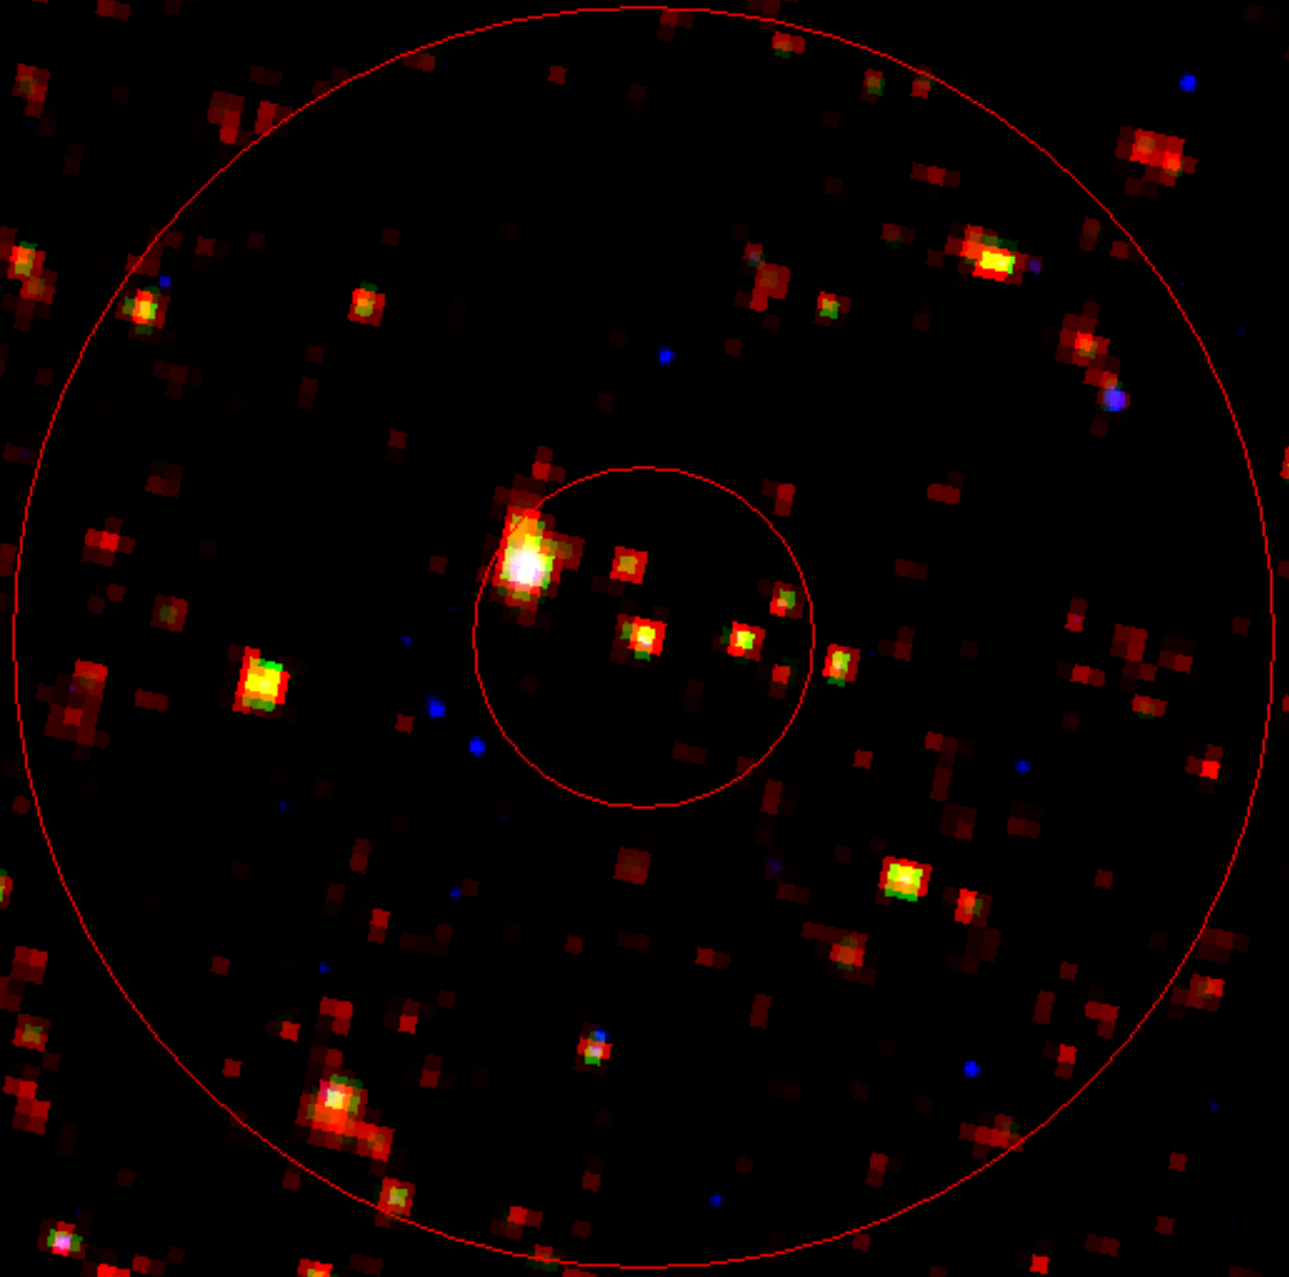}
            \\ RSG 4502 - 29 Myr
        \end{minipage}
        \begin{minipage}{.3\textwidth}
            \centering
            \includegraphics[width=\textwidth]{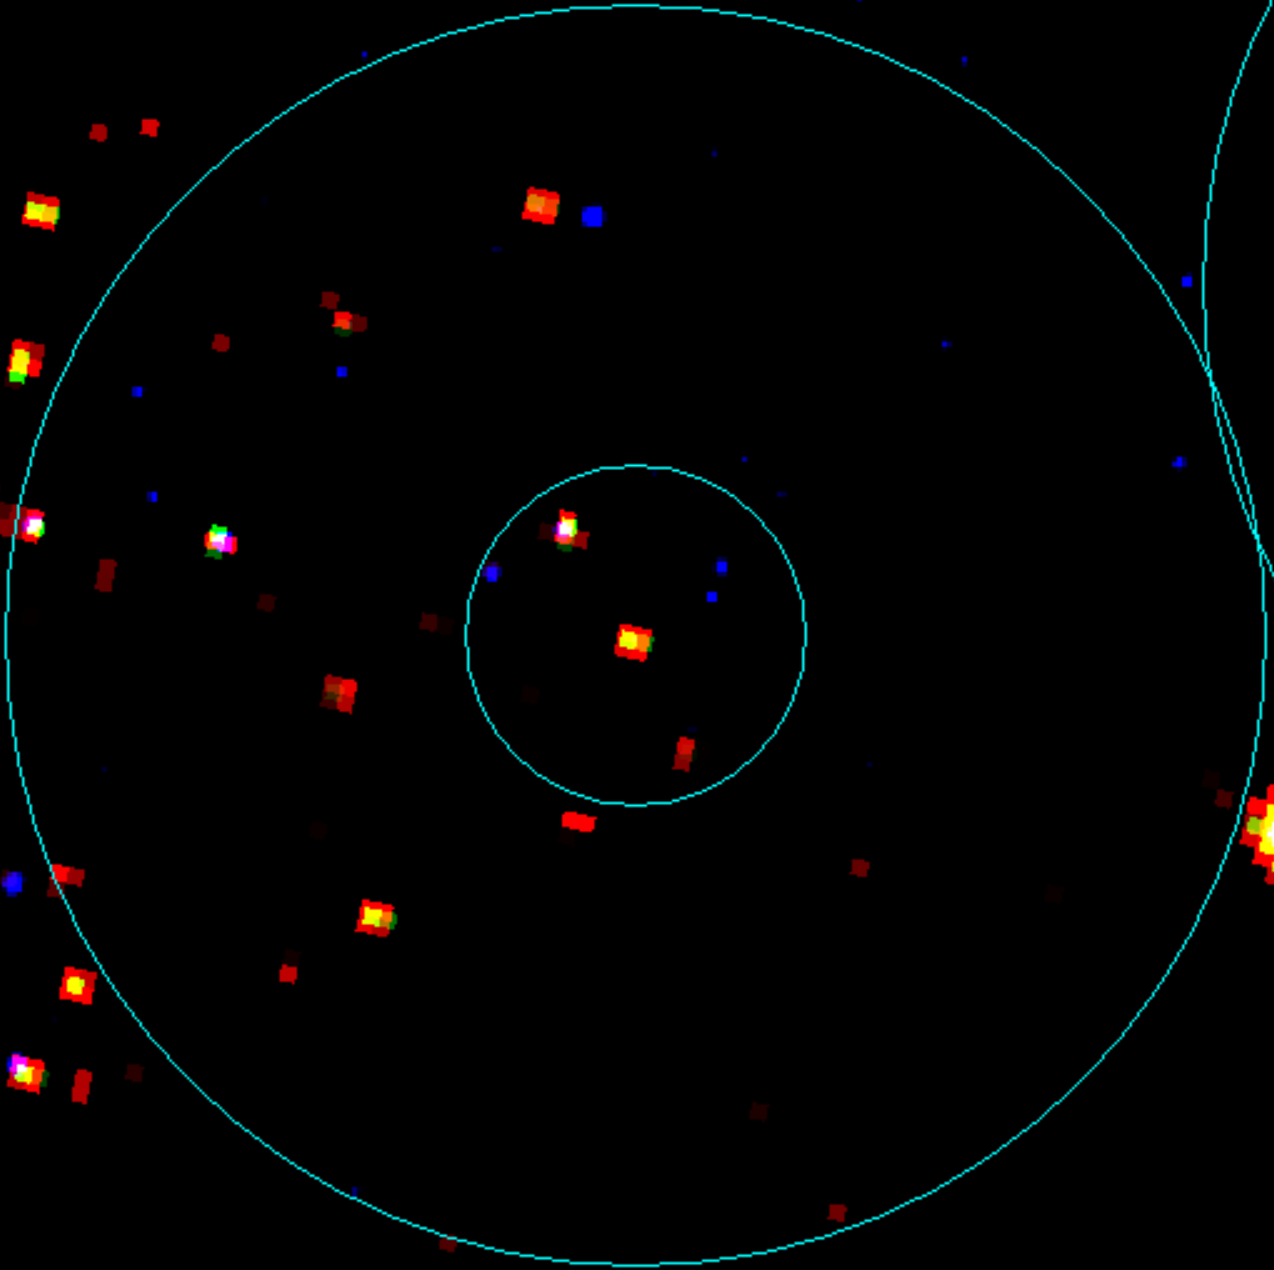}
            \\ RSG 4781 - 5 Myr
        \end{minipage}
        \begin{minipage}{.3\textwidth}
            \centering
            \includegraphics[width=\textwidth]{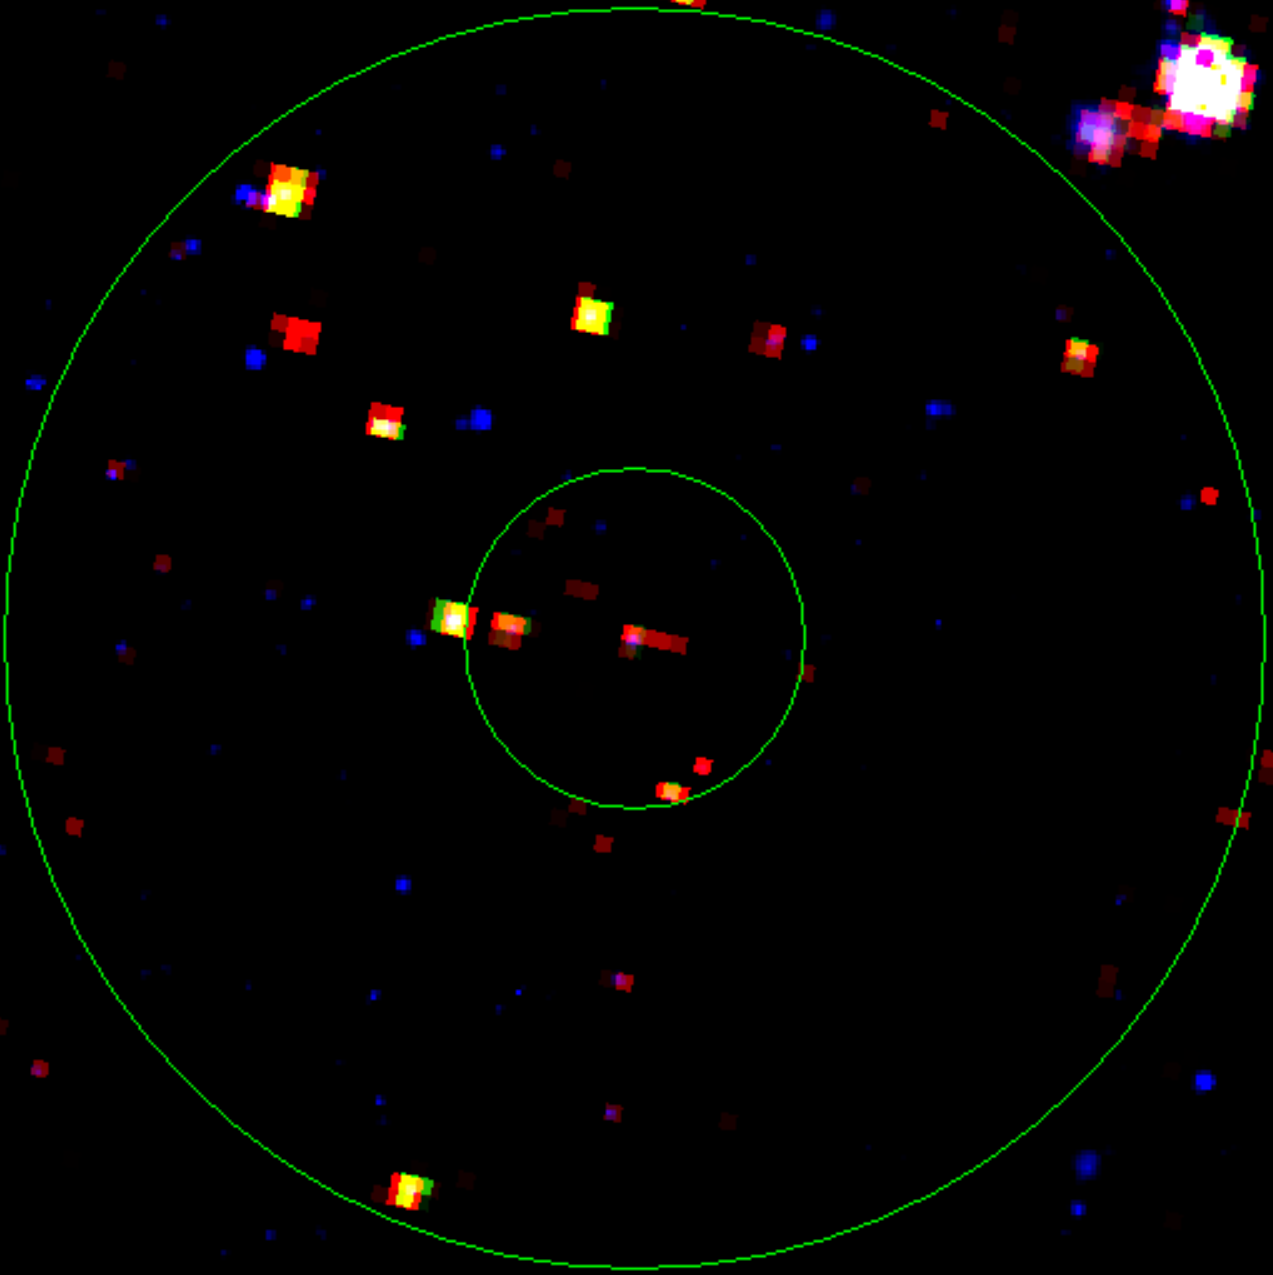}
            \\ RSG 5460 - 17 Myr
        \end{minipage}
        \begin{minipage}{.3\textwidth}
            \centering
            \includegraphics[width=\textwidth]{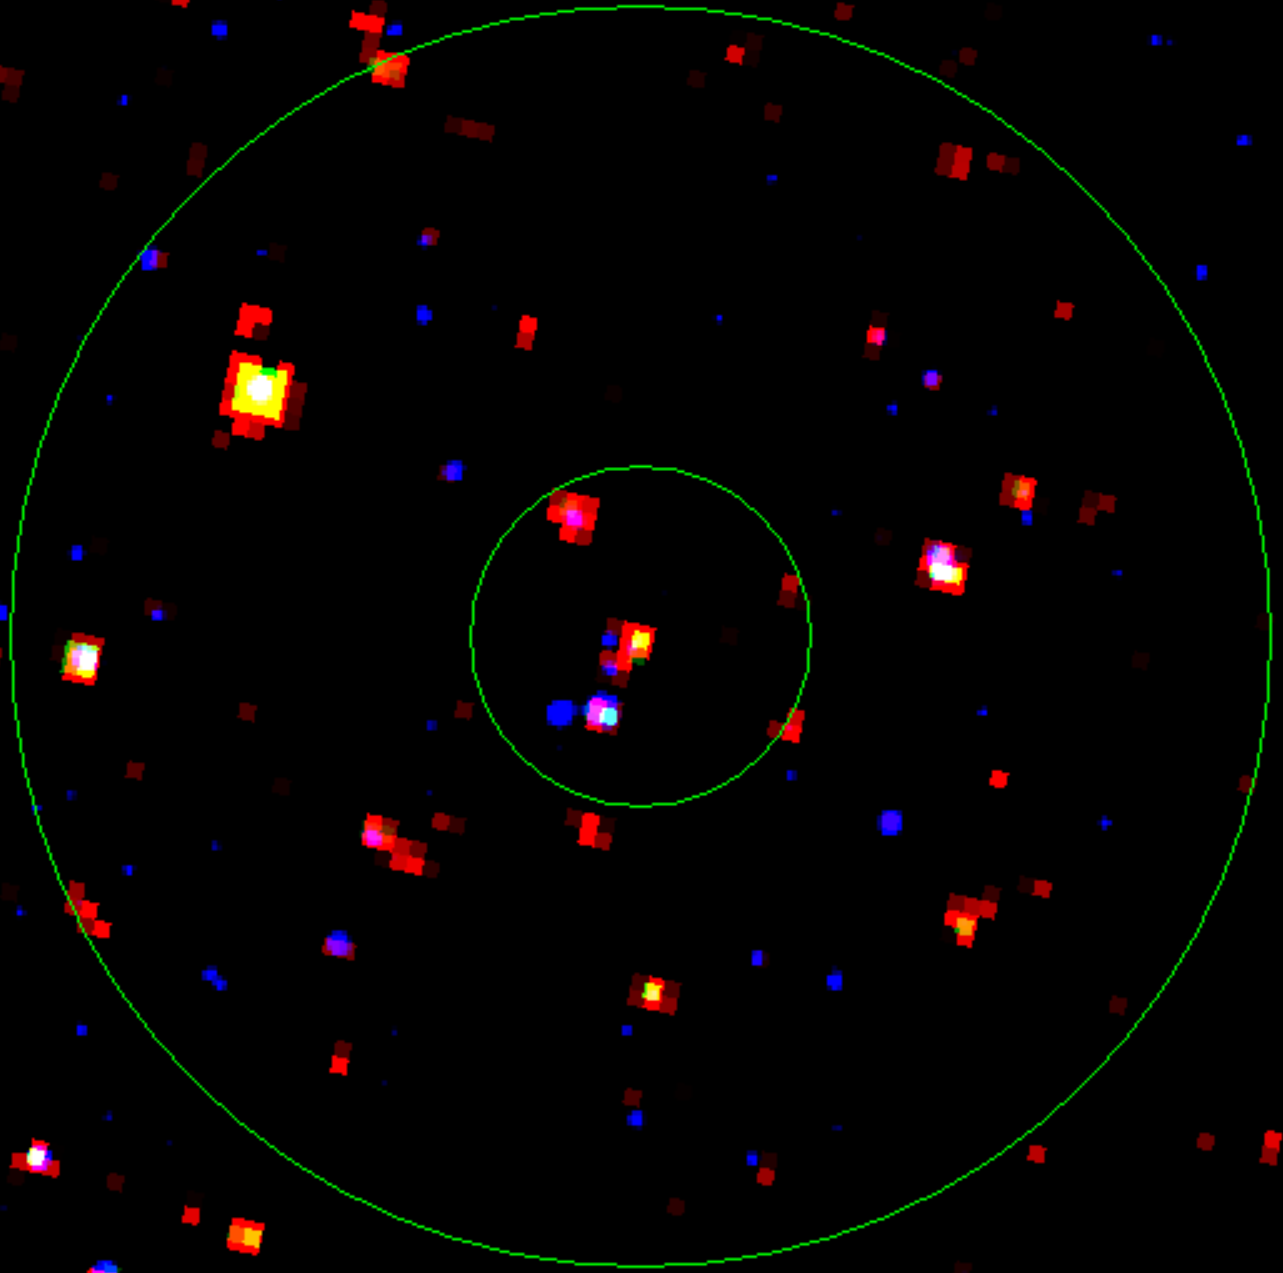}
            \\ RSG 3160 - 17 Myr
        \end{minipage}
        \begin{minipage}{.3\textwidth}
            \centering
            \includegraphics[width=\textwidth]{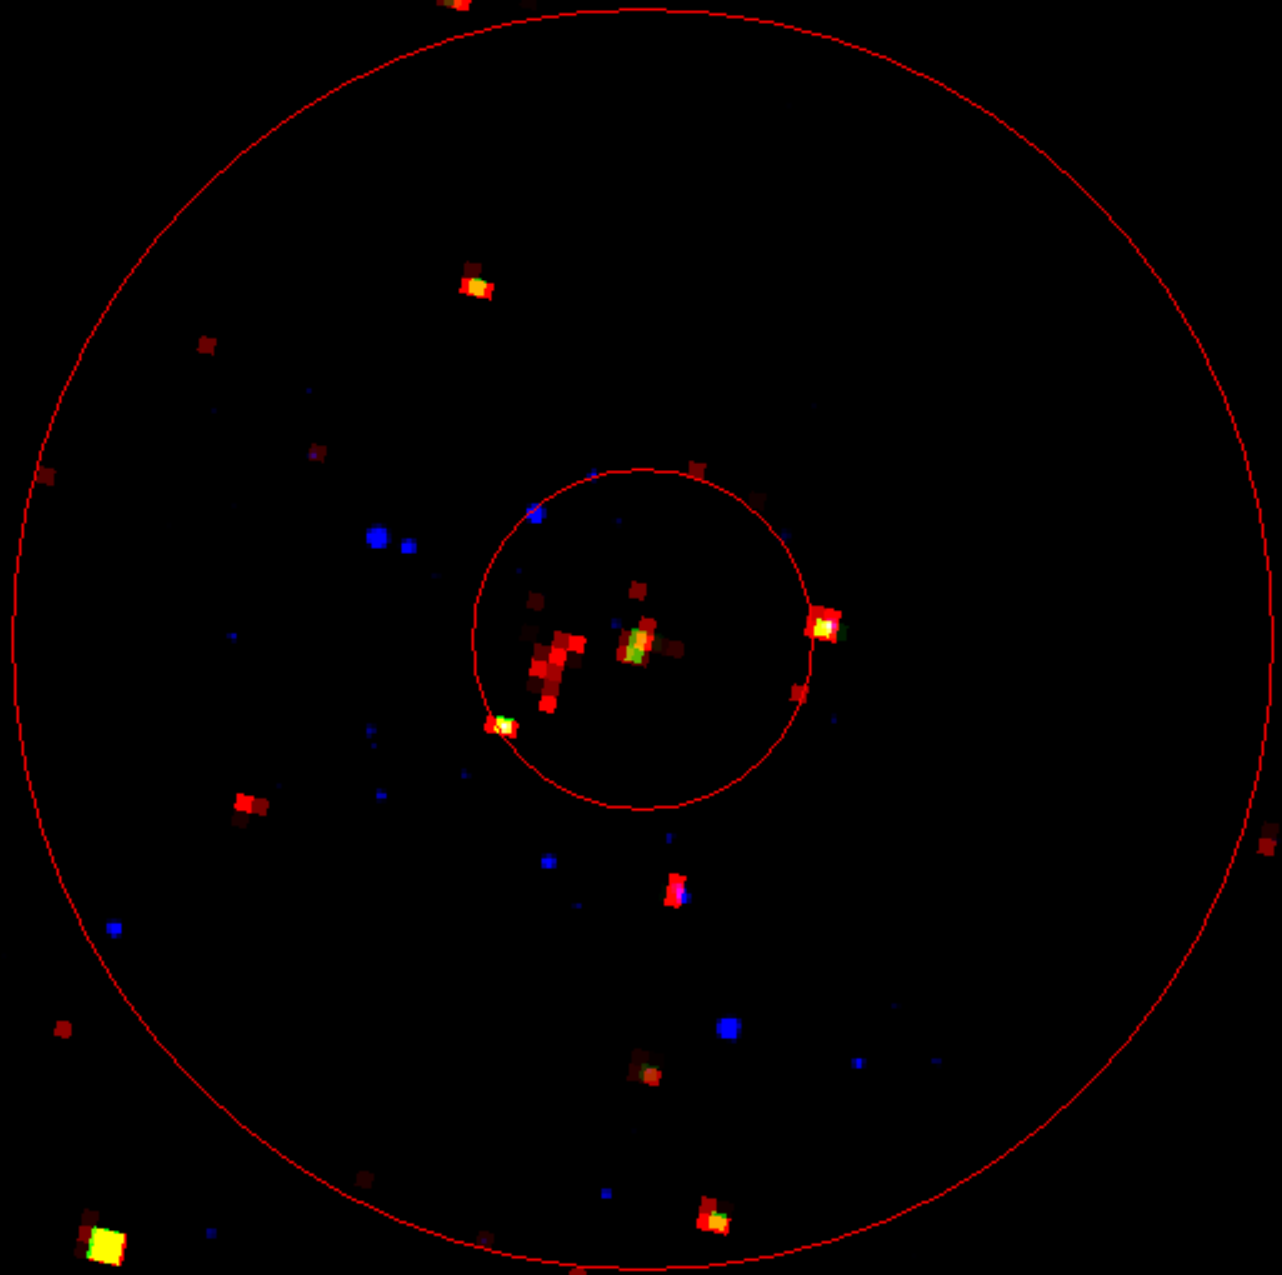}
            \\ RSG 2768 - 24 Myr
        \end{minipage}
        \begin{minipage}{.3\textwidth}
            \centering
            \includegraphics[width=\textwidth]{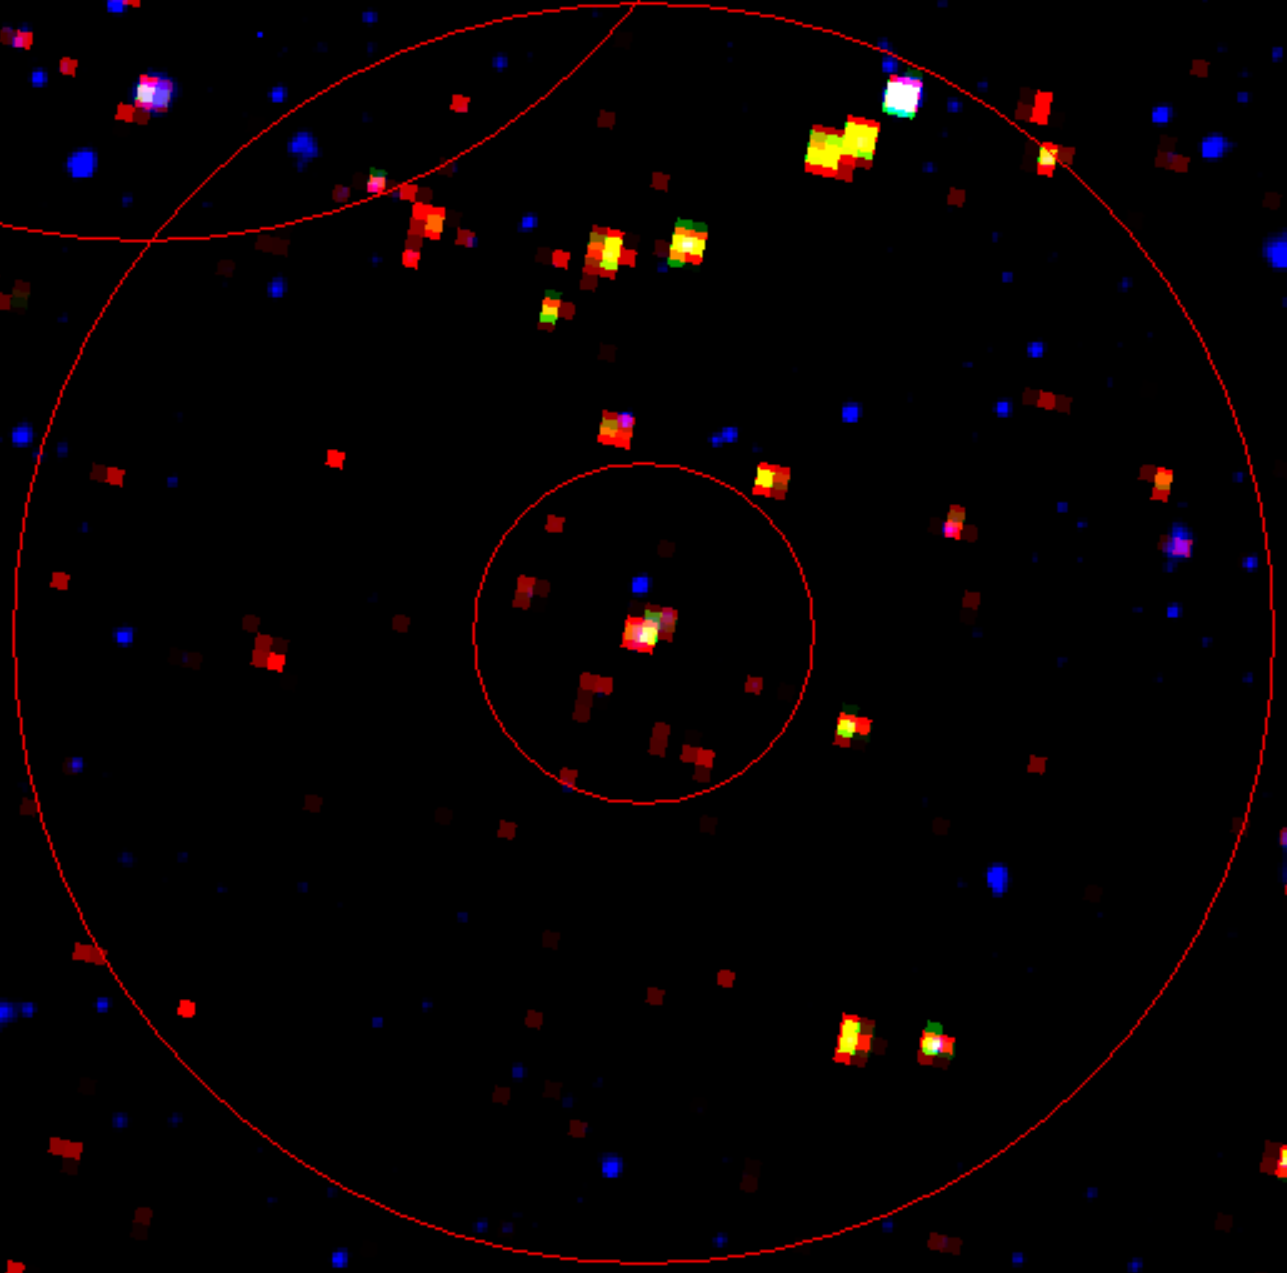}
            \\ RSG 3282 - 21 Myr
        \end{minipage}
        \begin{minipage}{.3\textwidth}
            \centering
            \includegraphics[width=\textwidth]{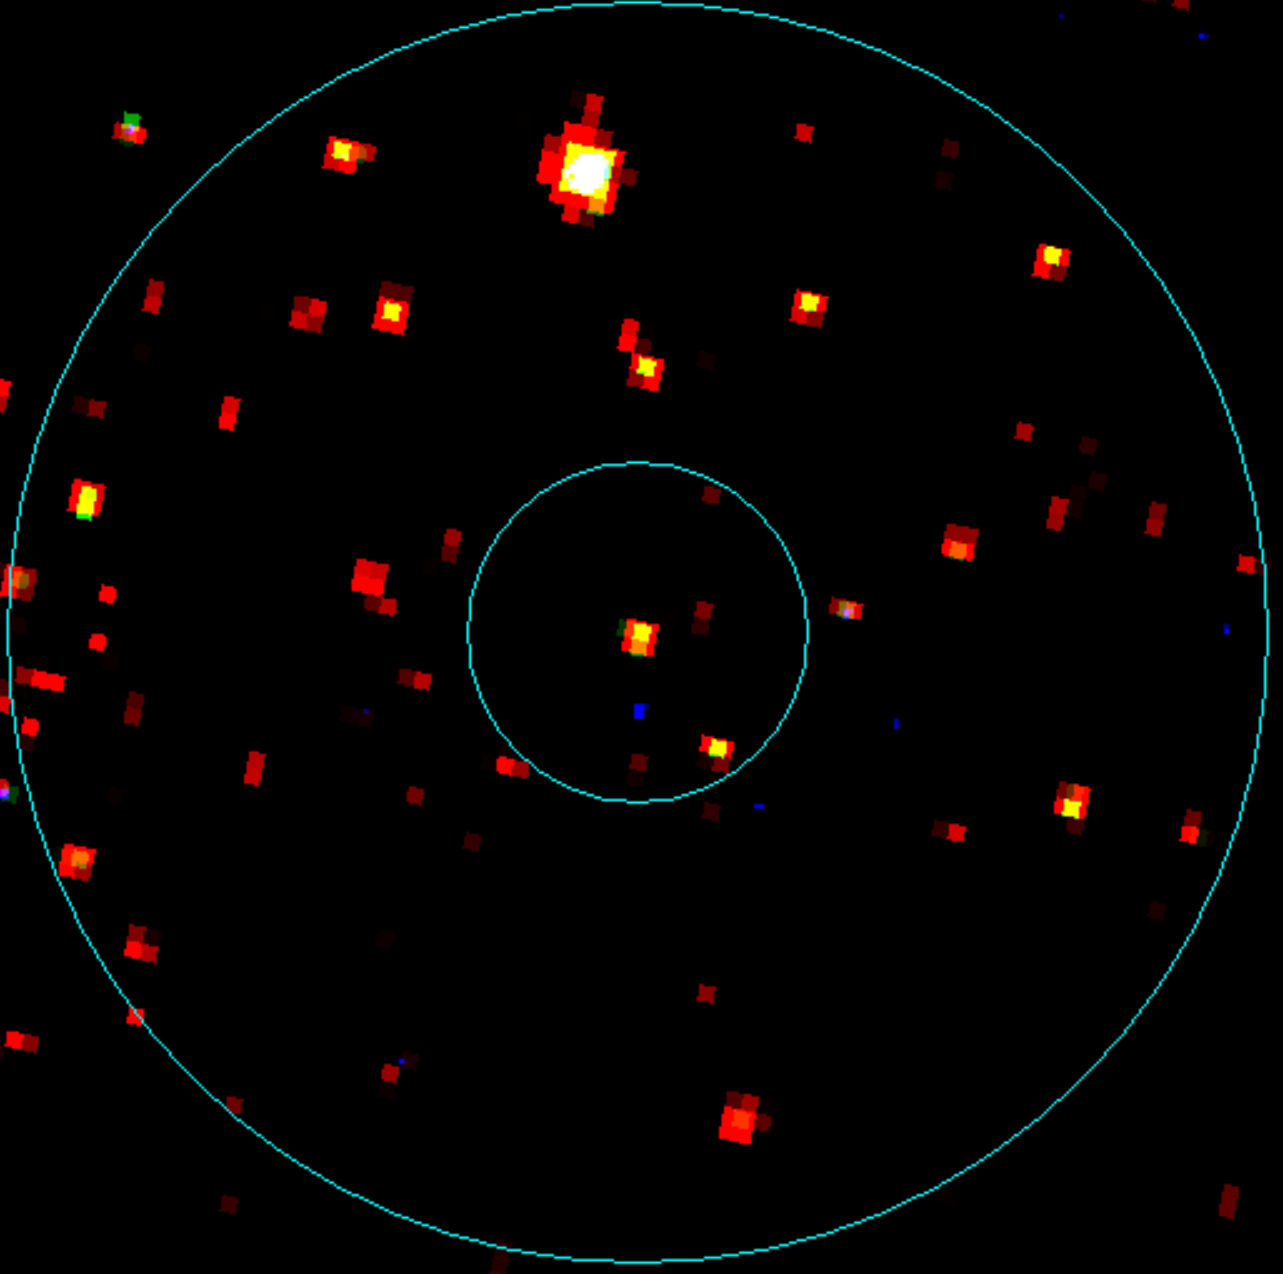}
            \\ RSG 3991 - 5 Myr
        \end{minipage}
        \begin{minipage}{.3\textwidth}
            \centering
            \includegraphics[width=\textwidth]{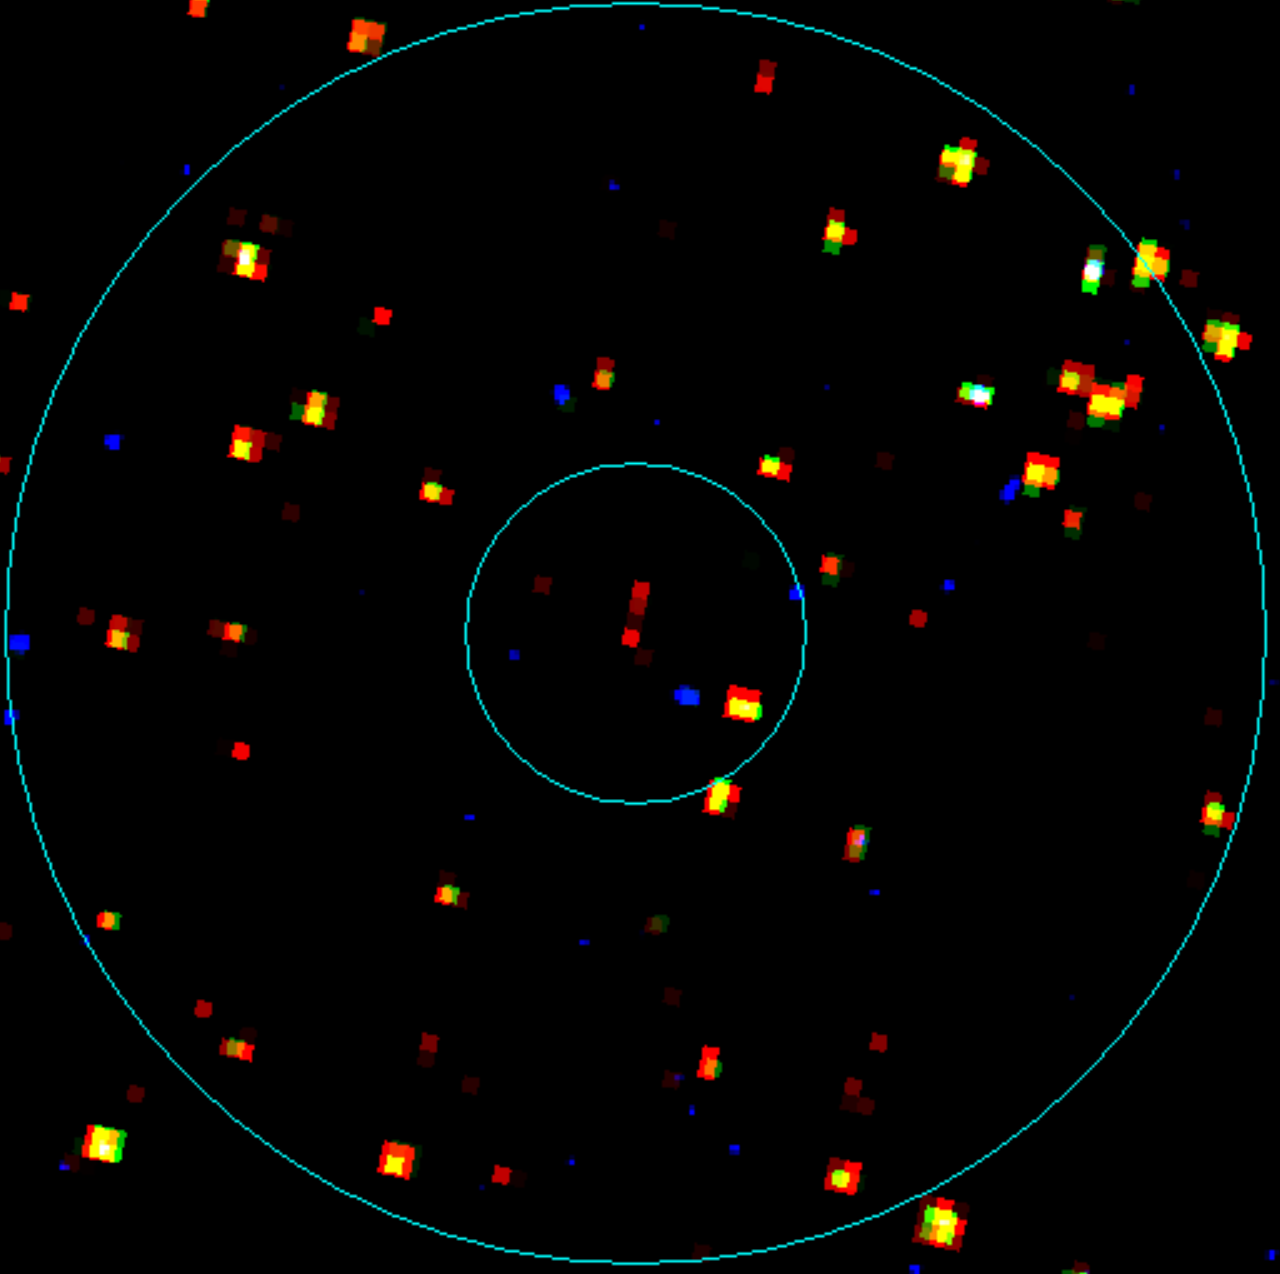}
            \\ RSG 2841 - 5 Myr
        \end{minipage}
    \end{figure}
